# Supplementary material for: Plug-and-Play Interpretable Responsible Text-to-Image Generation via Dual-Space Multi-facet Concept Control
Source: arXiv:2503.18324 source file (2025-03-24)
Supplement: Supplementary file 1 [file X_suppl.tex]

% \clearpage
% \appendix
% \setcounter{page}{1}
% % \setcounter{enumiv}{0} % Resets enumeration for citations
% \counterwithin{figure}{section}
% \counterwithin{table}{section}
\maketitlesupplementary

%\noindent {\Large \textbf{Appendix}}
\vspace{-2mm}

\noindent This  document provides detailed supplementary information to further explain the proposed framework and achieved results. %, it provides implementation details, and further results presented. 
It includes explanation of the training setup, algorithms, and technical specifics of the text embedding  and diffusion latent manipulations, which form the core of our dual-space technique. It extends the analysis with further experiments, ablation studies, and implementation guidelines to ensure  reproducibility. Our code can be accessed at \textcolor{magenta}{https://basim-azam.github.io/responsiblediffusion/}
\vspace{-3mm}
%%%%%%%%%%%%%%%%%%%%%%%%%%%%%%%%%%%%%%%%%%%%%%%%%%%%%%%%%%%%%%%%%%%%
\section{Further Algorithmic and Training Details}\label{A}
\vspace{-1mm}

We explore the proposed technique at two intervention points in text-to-image generative pipeline; namely, at  the text embedding space and the  diffusion latent space. Below, we provide further training details of our modules used for each of these points. 

\vspace{0.7mm}
\noindent \textbf{Training RICE Module:} Algorithm~\ref{alg:RICE} presents an overview of the training procedure of RICE module, which distills the teacher encoder module $\mathcal{E}(\cdot)$ into the student encoder module $\mathcal{E}_{resp}(\cdot)$, to produce $z_{clip}^{distill}$. The underlying model for the RICE module ($\psi_{\mathcal{E}}$) is built upon the CLIP text encoder model. This encoder processes tokenized text input into embeddings of shape $77 \times 768$, where the former represents the maximum sequence length and the latter is the dimensionality of each token's embedding. The architecture of our model comprises a 12-layer Transformer with 8 attention heads per layer, facilitating the generation of contextualized token embeddings. To align these embeddings with the responsible concept space $\mathcal{A}_{resp}$, the module incorporates distillation process, where the pre-trained CLIP model serves as the teacher. A knowledge distillation loss $\mathcal{L}_{KD-clip}$ minimizes the discrepancy between the teacher's embeddings and those of the student model.  Additionally, a whitening transformation generates $z^{zca}$, combined with $z^{distill}_{clip}$ using a weighting factor $\alpha$, yielding $z^{resp}_{clip}$. Backpropagation optimizes $\psi_{\mathcal{E}}$ iteratively across epochs and batches. This design ensure that the $\psi_{\mathcal{E}}$ integrates seamlessly in the T2I pipeline as a plug-in module for the generation of responsible images.

% Algorithm 1: Responsible and Interpretable CLIP Embeddings (RICE)
\begin{algorithm}[b]
\small
\caption{\small Responsible and Interpretable CLIP Embeddings}
\label{alg:RICE}
\textbf{Input:} Text Encoder $\mathcal{E}(\cdot)$, Concept Set $A_{X}$, Text Prompts $\mathcal{T}$, Batch Size $B$, Number of Epochs $N$ \\
\textbf{Output:} Trained RICE Module $\psi_{\mathcal E}$
\begin{algorithmic}[1]
    \State Initialize $\psi_{\mathcal E}$ and optimizer
    \For{\text{epoch} $= 1$ to $N$}
        \For{each batch $B \subset \mathcal{T}$}
            \State $z_{clip}^T = \mathcal{E}(B)$ \% Teacher Embeddings
            \State $z_{clip}^{distill} = \psi_{\mathcal E}(B)$ \% Student Embeddings
            \State 
            \[
            \mathcal{L}_{KD-clip} = \frac{1}{|B|} \sum_{k=1}^{|B|} \| z^T_{clip,k} - z^{distill}_{clip,k} \|^2
            \]
            \State 
            \[
            z^{zca} = \mathcal{W}(z^{distill}_{clip} - \mu), \quad \mu = \frac{1}{|B|} \sum_{k \in B} z^{distill}_{clip,k}
            \]
            \State
            \[
            z^{resp}_{clip} = \alpha z^{distill}_{clip} + (1 - \alpha) z^{zca}_{clip}
            \]
            \State Update $\psi_{\mathcal E}$
        \EndFor
    \EndFor
    \State \textbf{Return:} Trained $\psi_{\mathcal E}$
\end{algorithmic}
\end{algorithm}

\vspace{0.7mm}
\noindent \textbf{Training RIIDL Module:} Algorithm~\ref{alg:RIIDL} describes the training process for the RIIDL module with the underlying model \(\psi_{\mathcal{D}}\) whose architecture is inspired  by the U-Net structure of the Stable Diffusion v1.4. Our  U-Net model consists of a downsampling path with 4 stages, each including \(3 \times 3\) convolutional layers, group normalization, Swish activation, and residual connections. Downsampling reduces spatial resolution while progressively increasing feature channels, starting from 320 and doubling to 640, 1280, and 1280 across the stages. The bottleneck incorporates multi-head attention and residual blocks to capture global context and integrate cross-attention with text-conditioning inputs from the text encoder $\mathcal{E}(\cdot)$. %(\(77 \times 768\)). 
The upsampling path mirrors the downsampling structure, with transpose convolutions or bilinear upsampling to restore spatial resolution and skip connections to incorporate features from corresponding downsampling stages.

During training, the RIIDL module aligns the student's latents \(z_{\text{unet}}^{\text{distill},\tau}\) with the teacher's latents \(z_{\text{unet}}^{T,\tau}\) using a weighted distillation loss \(\mathcal{L}_{KD-unet}\). Intermediate latents are decorrelated through a whitening transformation, producing \(z_{\text{unet}}^{\text{zca},\tau}\). These transformed latents are then combined with \(z_{\text{unet}}^{\text{distill},\tau}\) using a weighting factor \(\beta\) to generate the composite latent \(z_{\text{unet}}^{\text{resp},\tau}\). The final refined latent aligns with \(\mathcal{A}_{\text{resp}}\) while preserving high-quality image generation. The RIIDL module’s design ensures responsibility-driven latent adjustments without altering the original U-Net's architecture, i.e  adaptation of $\Psi_{\mathcal{D}}$ as a plug-in module to produce responsible latents. 

\noindent \textbf{Dual Space Inference:} As we utilize both intervention points, i.e., text embedding space and the diffusion latent space, Algorithm~\ref{alg:dual_space} summarizes our dual-space inference process, harmonizing image generation while enforcing responsible aspects. The process  combines RICE ($\psi_{\mathcal E}$) refined text embeddings and RIIDL ($\psi_{\mathcal D}$) enhanced latents. Responsible embeddings $z_{clip}^{final}$ and latents $z_{unet}^{final}$ are fused into a unified representation using control weights $\lambda_{\mathcal E}$ and $\lambda_{\mathcal D}$  such that $\lambda_{\mathcal E} + \lambda_{\mathcal D} = 1$. The final image $\hat{I}$ adheres to $\mathcal{A}_{resp}$ while preserving the base T2I model's visual quality. The modular design keeps the pre-trained diffusion model unchanged, with RICE and RIIDL modules acting as external plug-ins in the T2I pipeline.

\vspace{0.7mm}
\noindent \textbf{Hyperparameter Settings:} 
\textcolor{black}{The hyperparameters $\alpha$ in RICE and the corresponding parameter $\beta$ in RIIDL balance semantic retention with responsibility aspects. They govern  control between embeddings or latents and their decorrelated counterparts, subtly reinforcing responsible alignments while maintaining semantic and visual precision. The values of $\alpha$ and $\beta$ are selected to give minimal but meaningful weight to the decorrelated components (i.e., 0.1). This ensures the influence without dominating the primary embeddings or latents. This value is empirically determined by inspecting visual quality of the outputs.  During inference, a dominant emphasis on text embeddings is ensured through  $\lambda_{\mathcal{E}} = 95\%$ for retaining the  original  semantics, while latent-space refinements via $\lambda_{\mathcal{D}} = 5\%$ is chosen to provide subtle enhancements that result in high image quality. All  hyperparameters $\alpha , \beta, \lambda_{\mathcal{E}}$, and $\lambda_{\mathcal{D}}$ are determined through iterative experimentation and empirical analysis, balancing their adaptation across diverse scenarios. This balance enables effective  module integration for RICE and RIIDL as plug-ins in the T2I pipeline for responsible image generation. }

\vspace{0.7mm}
\noindent \textbf{Training Setup:}  
In our experiments, we use Stable Diffusion v1.4 checkpoint as the base model with a guidance scale of 7.5 for high-quality image generation. Concept spaces \(\mathcal{A}_{race}\), \(\mathcal{A}_{age}\), and \(\mathcal{A}_{gender}\) are trained using 1,000 synthesized images per concept, optimized over 10,000 steps. During inference, these concept spaces are applied within the dual-space control framework to enforce adherence to \(\mathcal{A}_{resp}\). We empirically find that that higher values of \(\lambda_{\mathcal{D}}\) yield better results, emphasizing the importance of latent space interventions in maintaining structural fidelity while ensuring responsibility constraints.  The experiments are carried out on a single node of the an HPC system  equipped with 4 NVIDIA A100 GPUs (80GB each), 495GB of RAM, and 32 CPU cores. 
\begin{algorithm}[t]
\small
\caption{\small Responsible Interpretable Intermediate Diffusion Latents}
\label{alg:RIIDL}
\textbf{Input:} Diffusion Model $\mathcal{D}(\cdot)$, Concept Set $A_{X}$, Batch Size $B$, Number of Epochs $N$ \\
\textbf{Output:} Trained RIIDL Module $\psi_{\mathcal D}$
\begin{algorithmic}[1]
    \State Initialize $\psi_{\mathcal D}$ and optimizer
    \For{\text{epoch} $= 1$ to $N$}
        \For{each batch $B$}
            \State Uniformly sample time step $\tau \sim U[0, 1]$
            \State $z_{unet}^{T,\tau} = \mathcal{D(\mathcal{E}(\cdot))}$ \% Techer Latents
            \State $z_{unet}^{distill,\tau}$ = $\psi_{\mathcal D}(B)$ \% Student Latents
            \State 
            \[
            L_{KD-unet} = \omega(\lambda_\tau) \| z_{unet}^{T,\tau} - z_{unet}^{distill,\tau} \|^2
            \]
            \State 
            \[
            z_{unet}^{zca,\tau} = W(z_{unet}^{distill,\tau} - \mu)
            \]
            \State 
            \[
            z_{unet}^{resp,\tau} = \beta z_{unet}^{distill,\tau} + (1 - \beta) z_{unet}^{zca,\tau}
            \]
            \State Update $\psi_{\mathcal D}$
        \EndFor
    \EndFor
    \State \textbf{Return:} Trained $\psi_{\mathcal D}$
\end{algorithmic}
\end{algorithm}

% Algorithm 3: Dual-Space Integration and Inference Pipeline
\begin{algorithm}[ht]
\footnotesize
\caption{\small Dual-Space Integration and Inference Process}
\label{alg:dual_space}
\textbf{Input:} Text Prompt $t$, RICE Module $\psi_{\mathcal E}$, RIIDL Module $\psi_{\mathcal D}$, T2I Model $\Psi$, Weights $\lambda_{\mathcal E}$, $\lambda_{\mathcal D}$ \\
\textbf{Output:} Responsible Image $\hat{I}$
\begin{algorithmic}[1]
    \State Compute original text embeddings:
    \[
    z_{clip} = \mathcal{E}(t)
    \]
    \State Compute responsible embeddings using RICE:
    \[
    z_{clip}^{final} = z_{clip} + \sum_k \gamma_k z_{k,clip}^{resp}
    \]
    \State Define the responsible embedding module:
    \[
    \Psi_{\mathcal{E}} = \mathcal{E}_{resp}(t), \quad \text{where } \mathcal{E}_{resp} \text{ uses } z_{clip}^{final}
    \]
    \State Compute original latent representation using the diffusion model:
    \[
    z_{unet} = \mathcal{D}(\mathcal{E}(t))
    \]
    \State Compute responsible latents using RIIDL:
    \[
    z_{unet}^{final} = z_{unet} + \sum_k \gamma_k z_{k,clip}^{resp}
    \]
    \State Define the responsible latent module:
    \[
    \Psi_{\mathcal{D}} = \mathcal{D}_{resp}(\mathcal{E}(t)), \quad \text{where } \mathcal{D}_{resp} \text{ uses } z_{unet}^{final}
    \]
    \State Combine embedding and latent representations via dual-space control:
    \[
    \Psi_{resp}(t) = \lambda_{\mathcal E} \Psi_{\mathcal{E}} + \lambda_{\mathcal D} \Psi_{\mathcal{D}}, \quad \lambda_{\mathcal E} + \lambda_{\mathcal D} = 1
    \]
    \State Generate the final responsible image:
    \[
    \hat{I} = \Psi_{resp}(t)
    \]
    \State \textbf{Return:} Responsible Image $\hat{I}$
\end{algorithmic}
\end{algorithm}

\section{Further Results}
In the main paper, we analyzed the dual-space control framework's effectiveness in mitigating biases across professions using  WinoBias dataset~\cite{zhao2018gender}, as detailed in sections 5 and 6 of the paper. To extend the analysis we provide additional results to demonstrate further capabilities of our framework here. 

Figures~\ref{fig:sd_ours} and~\ref{fig:composite_supp} provide further examples of successful control over responsible concepts using our technique.  Figure~\ref{fig:sd_ours} provides a pairwise comparison of baseline Stable Diffusion (SD) and our responsible generation outputs, where baseline outputs often reflect stereotypical associations. By incorporating our technique, the generation aligns  with the responsible concept space $\mathcal{A}_{X}$. This alignment ensures balanced and non-stereotypical representations across the professions. Figure~\ref{fig:composite_supp} presents the ability of the  proposed approach to incorporate different responsible attributes of age, gender and race in the generated content for different professions.  
%to generate diverse outputs across several professions, demonstrating control over age, gender, and race attributes. 
Figure~\ref{fig:composite_supp_2} extends this analysis by incorporating multiple aspects from different concepts simultaneously to generate responsible outputs. It is observable that the generated outputs remain  high-quality and they preserve the original semantics while incorporating the multi-facet responsible concepts that we like to be considered in the outputs. This is a key strength of our method. 

%to composite scenarios, showing the framework’s ability to integrate multiple concept aspects simultaneously.

In section 6 of the main paper, we presented curtailed results about the transitions caused by RICE and RIIDL modules. Figures~\ref{fig:embeddings_interpolation} and~\ref{fig:latent_interpolation} provide extended results for the same purpose.  The results emphasize the roles of RICE and RIIDL modules in enabling fine-grained control. Figure~\ref{fig:embeddings_interpolation} demonstrates smooth interpolation within the embedding space, transitioning across attributes such as gender and race, with corner anchor images representing distinct combinations. Figure~\ref{fig:latent_interpolation} highlights RIIDL's ability to refine latent space representations during diffusion, aligning outputs with responsible attributes at various denoising steps. Additional examples in Figures~\ref{fig:Ng1} and~\ref{fig:Ng2} exhibit the further scalability of our framework. Figure~\ref{fig:Ng1} integrates additional attributes (e.g., smile, glasses) into professional contexts, while Figure~\ref{fig:Ng2} extends the approach to abstract prompts such as animals and activities (e.g., “a dog skateboarding”). These results validate the versatility and adaptability of the proposed method across diverse cases.

In the main paper, we presented quantitative results 
on Winobias dataset to quantify bias and debiasing for randomly selected classes (due to space restrictions). Here, Tables~\ref{tab:supp_fairness} and~\ref{tab:merged_debiasing_performance} present extensive   results along the same lines to demonstrate the efficacy of the proposed framework against prior works. Table~\ref{tab:supp_fairness} reports deviation ratio values (\(\Delta\)) across gender and racial attributes, showing that our method achieves the lowest average deviation across all attributes, outperforming standard Stable Diffusion and competing methods such as Unified Concept Editing (U)~\cite{gandikota2024unified} and Vector Interpret Diffusion (V)~\cite{li2024self}. Table~\ref{tab:merged_debiasing_performance} further corroborates these findings by presenting debiasing performance results, where our approach achieves the lowest average deviation, indicating superior fairness.

% \section*{Acknowledgment}
% This research was supported by The University of Melbourne’s Research Computing Services and the Petascale Campus Initiative.
%NA: Its double blind, we can not give any information about ourselves or university.

%%%%%%%%%%%%%%%%%%%%%%%%%%%%%%%%%%%%%%%%%%%%%%%%%%%%%%%%%%%%%%%%%%%%

\begin{figure*}
    \centering
    \includegraphics[width=\linewidth]{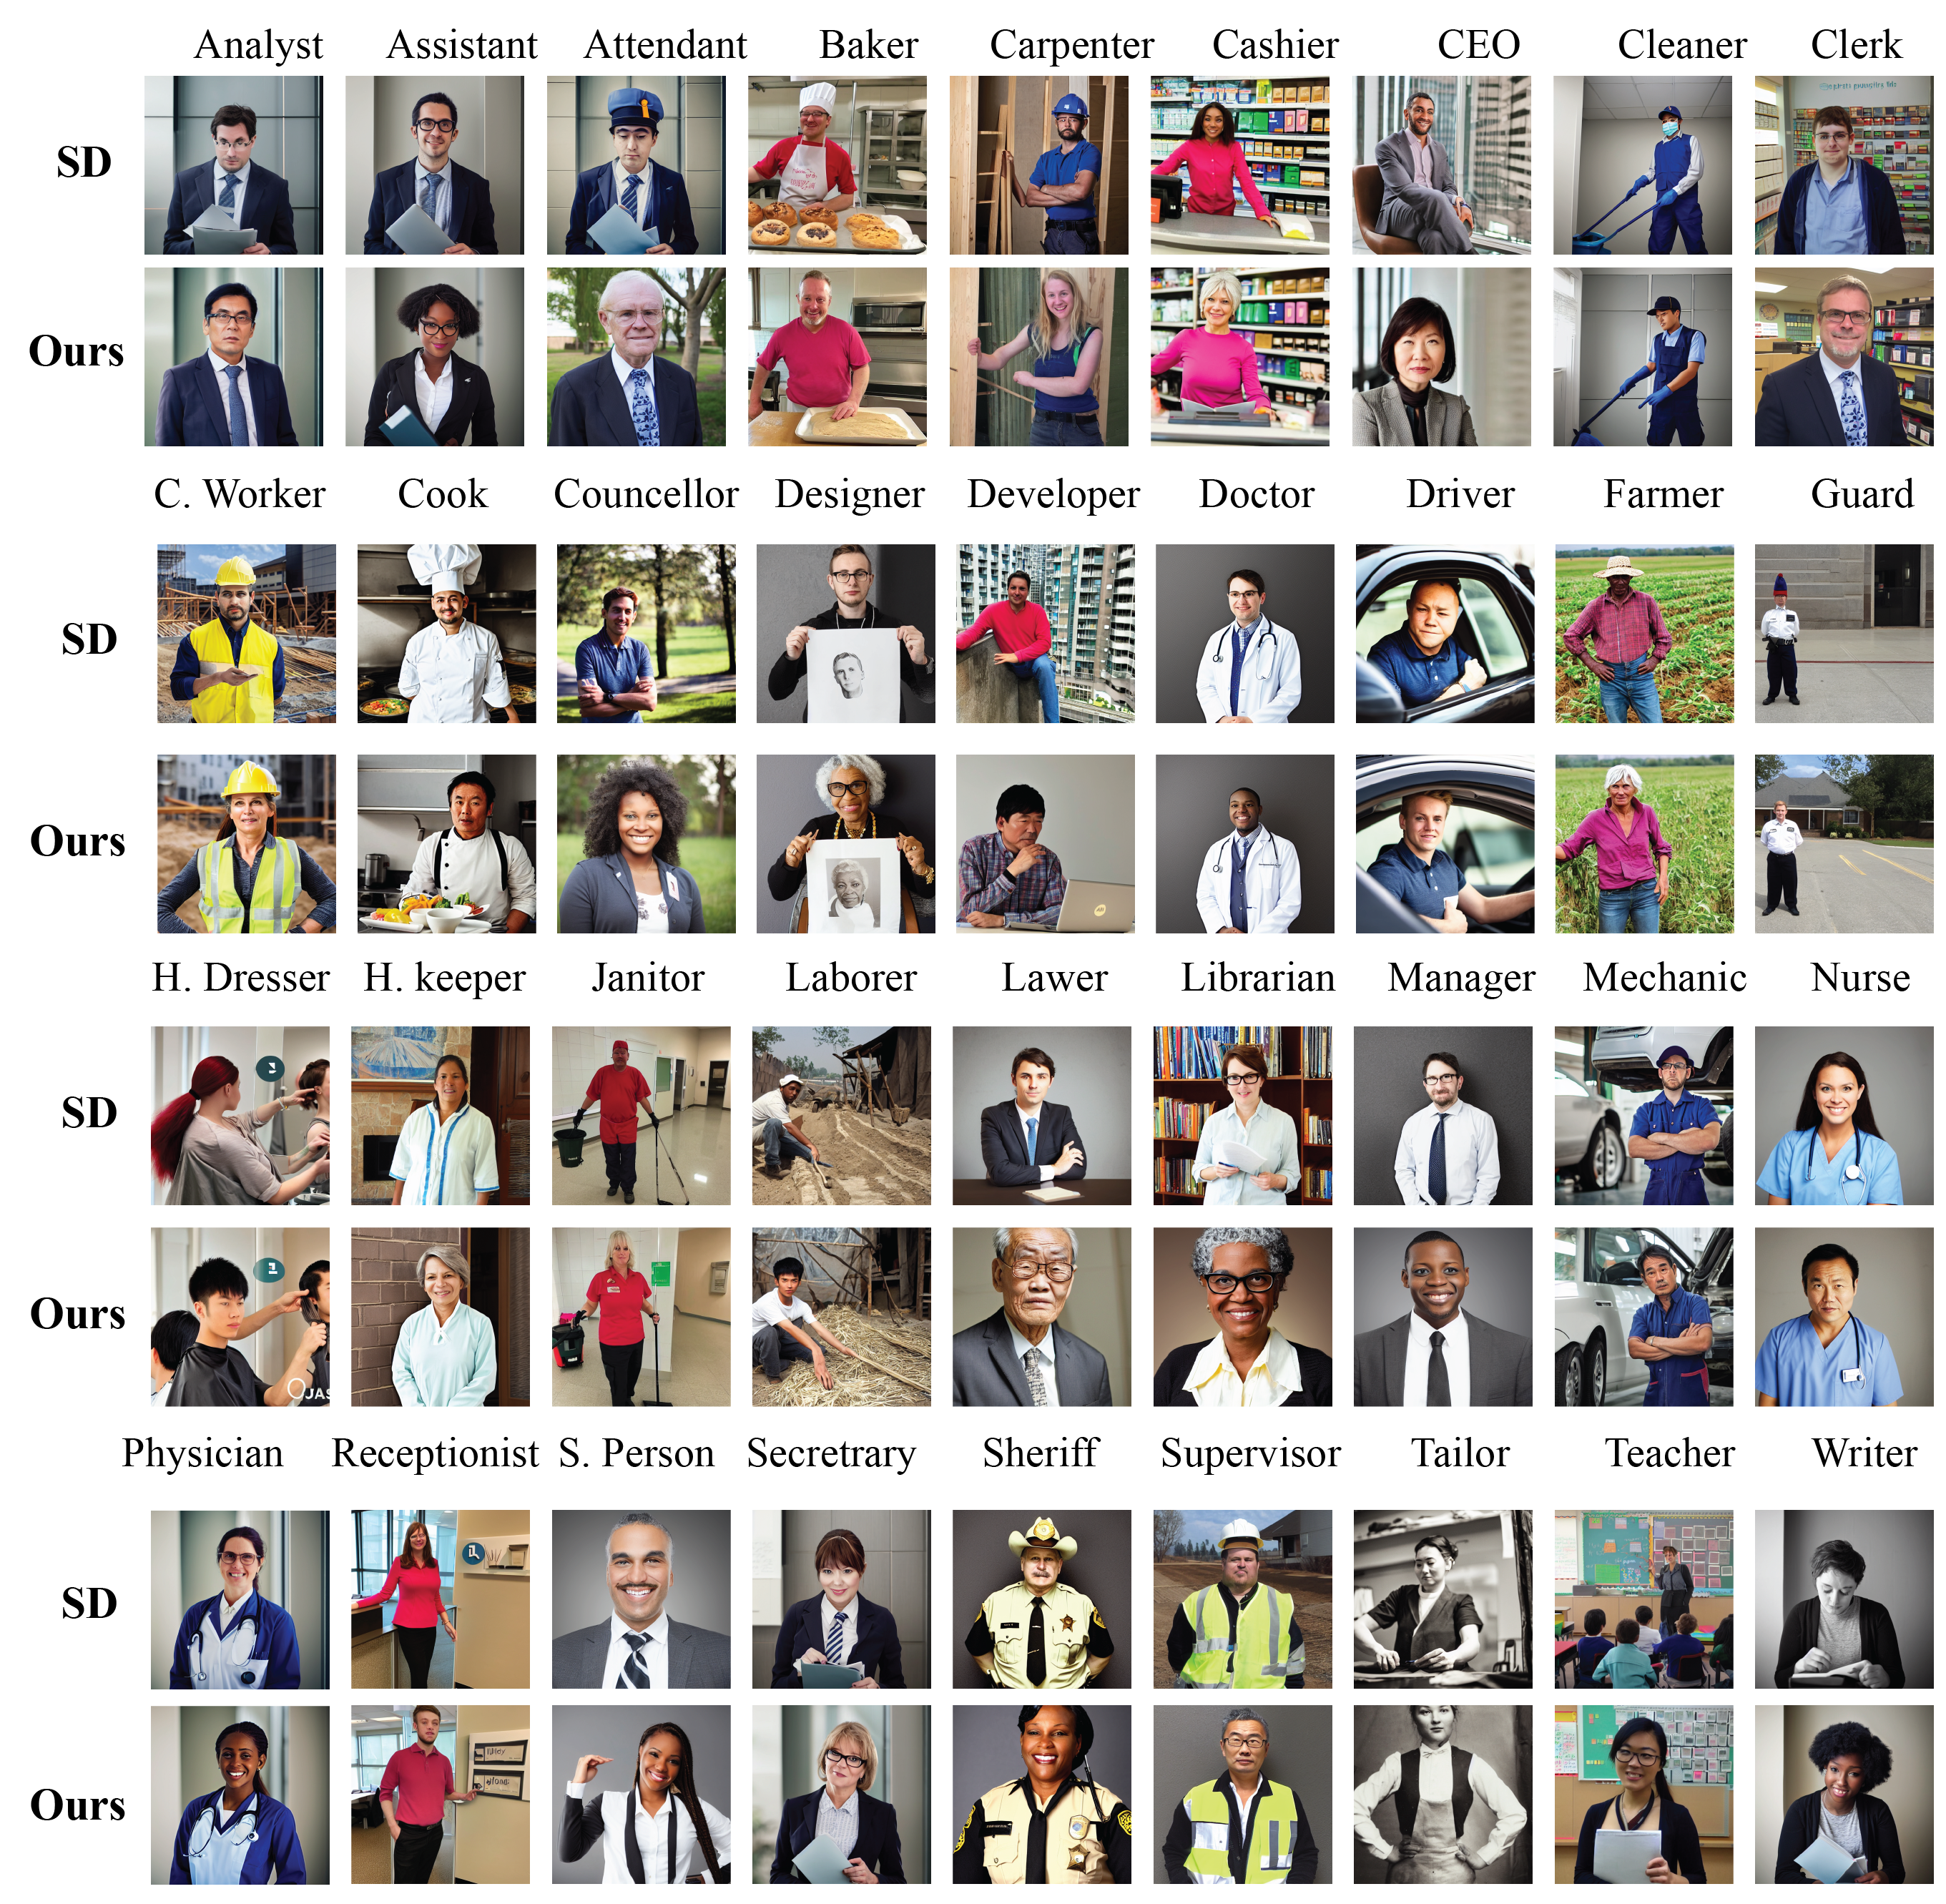}
    \caption{Pairwise Comparison of Baseline and Responsible Generation Outputs. 
Each pair  compares Stable Diffusion (SD) outputs (top) with our responsible generation plugin (bottom) across age, gender, and race attributes for each profession in Winobias \cite{zhao2018gender} dataset. SD outputs often show stereotypical biases, such as gender or racial associations among the professions. Using our technique, incorporating $\psi_\mathcal{E}$  and $\psi_\mathcal{D}$, these biases are mitigated by aligning outputs with responsible aspects. Our method ensures fair, diverse, and high-quality generation while removing harmful stereotypes.}
    \label{fig:sd_ours}
\end{figure*}

\begin{figure*}
    \centering
    \includegraphics[width=\linewidth]{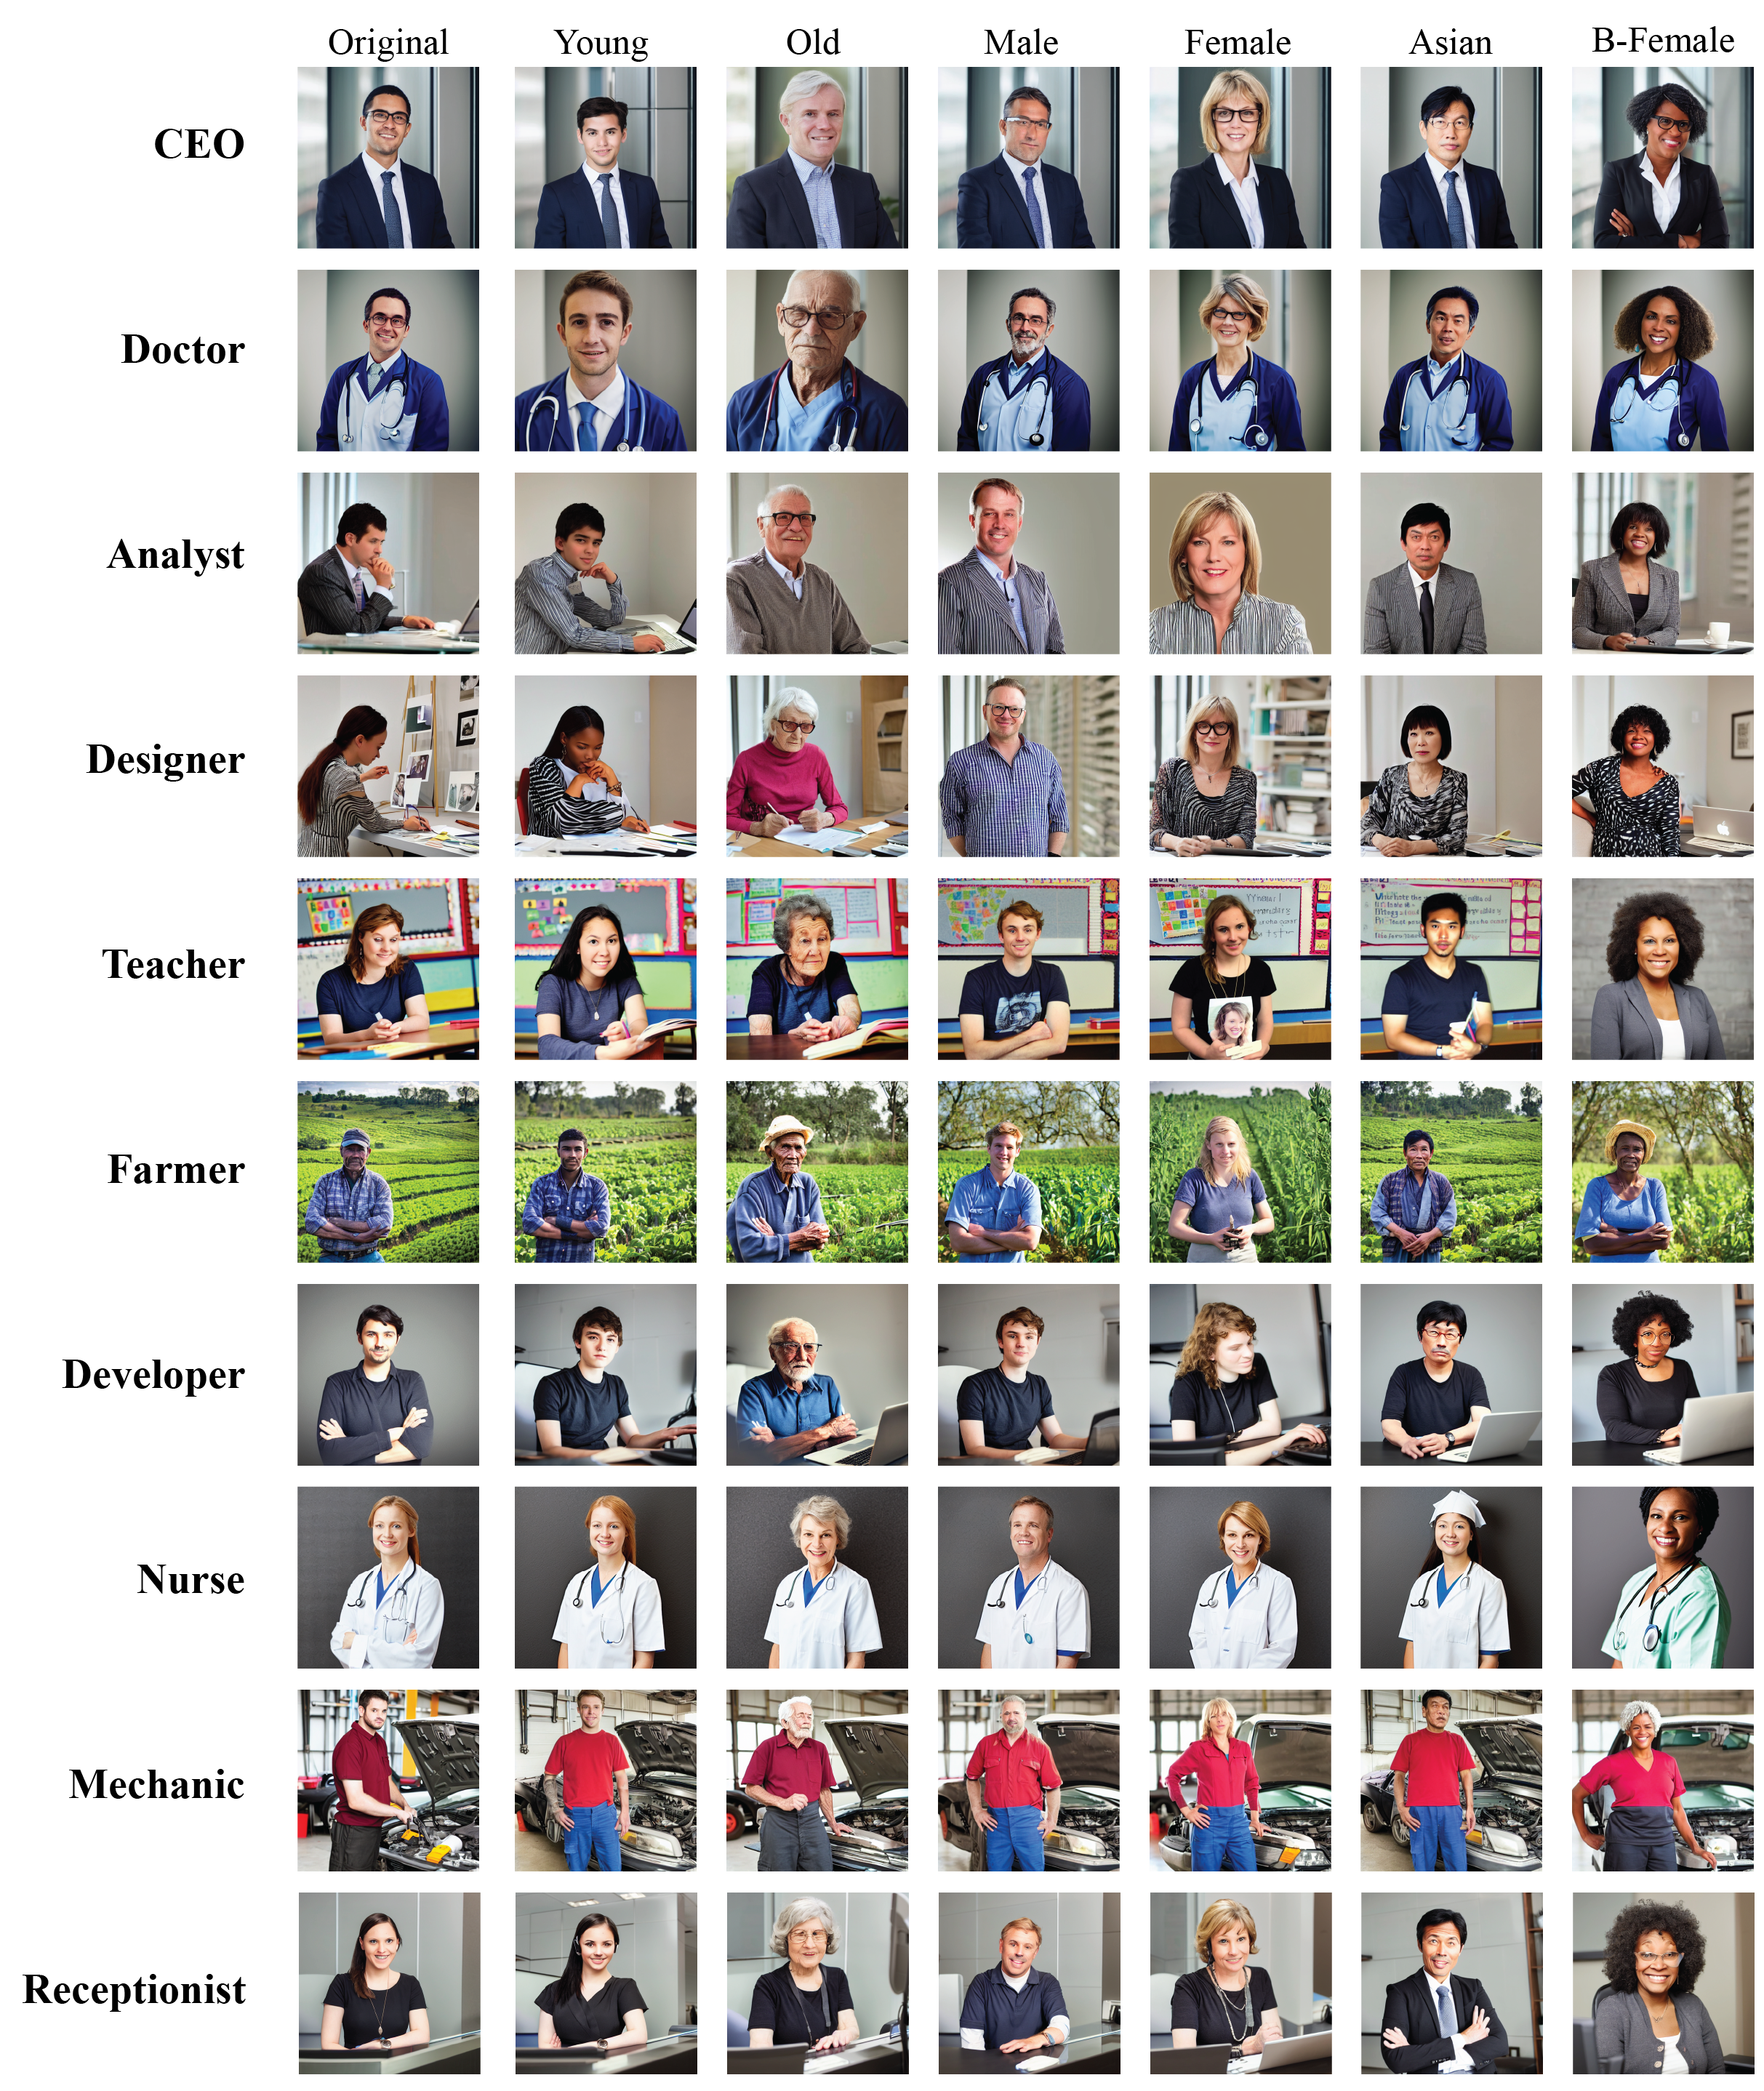}
    \caption{Controlled responsible generation by incorporating different individual concepts in the outputs. The figure showcases  images generated by incorporating our technique into Stable Diffusion with individual control over attributes such as age, gender, and race. The prompt "A <profession-name>" is used to generate the image, and individual target concept space from ($\mathcal{A}_X$) is plugged in using the proposed approach. Each row highlights selected profession from the Winobias dataset \cite{zhao2018gender}, while columns represent the incorporation of concept spaces.}
    \label{fig:composite_supp}
\end{figure*}

\begin{figure*}
    \centering
    \includegraphics[width=0.95\linewidth]{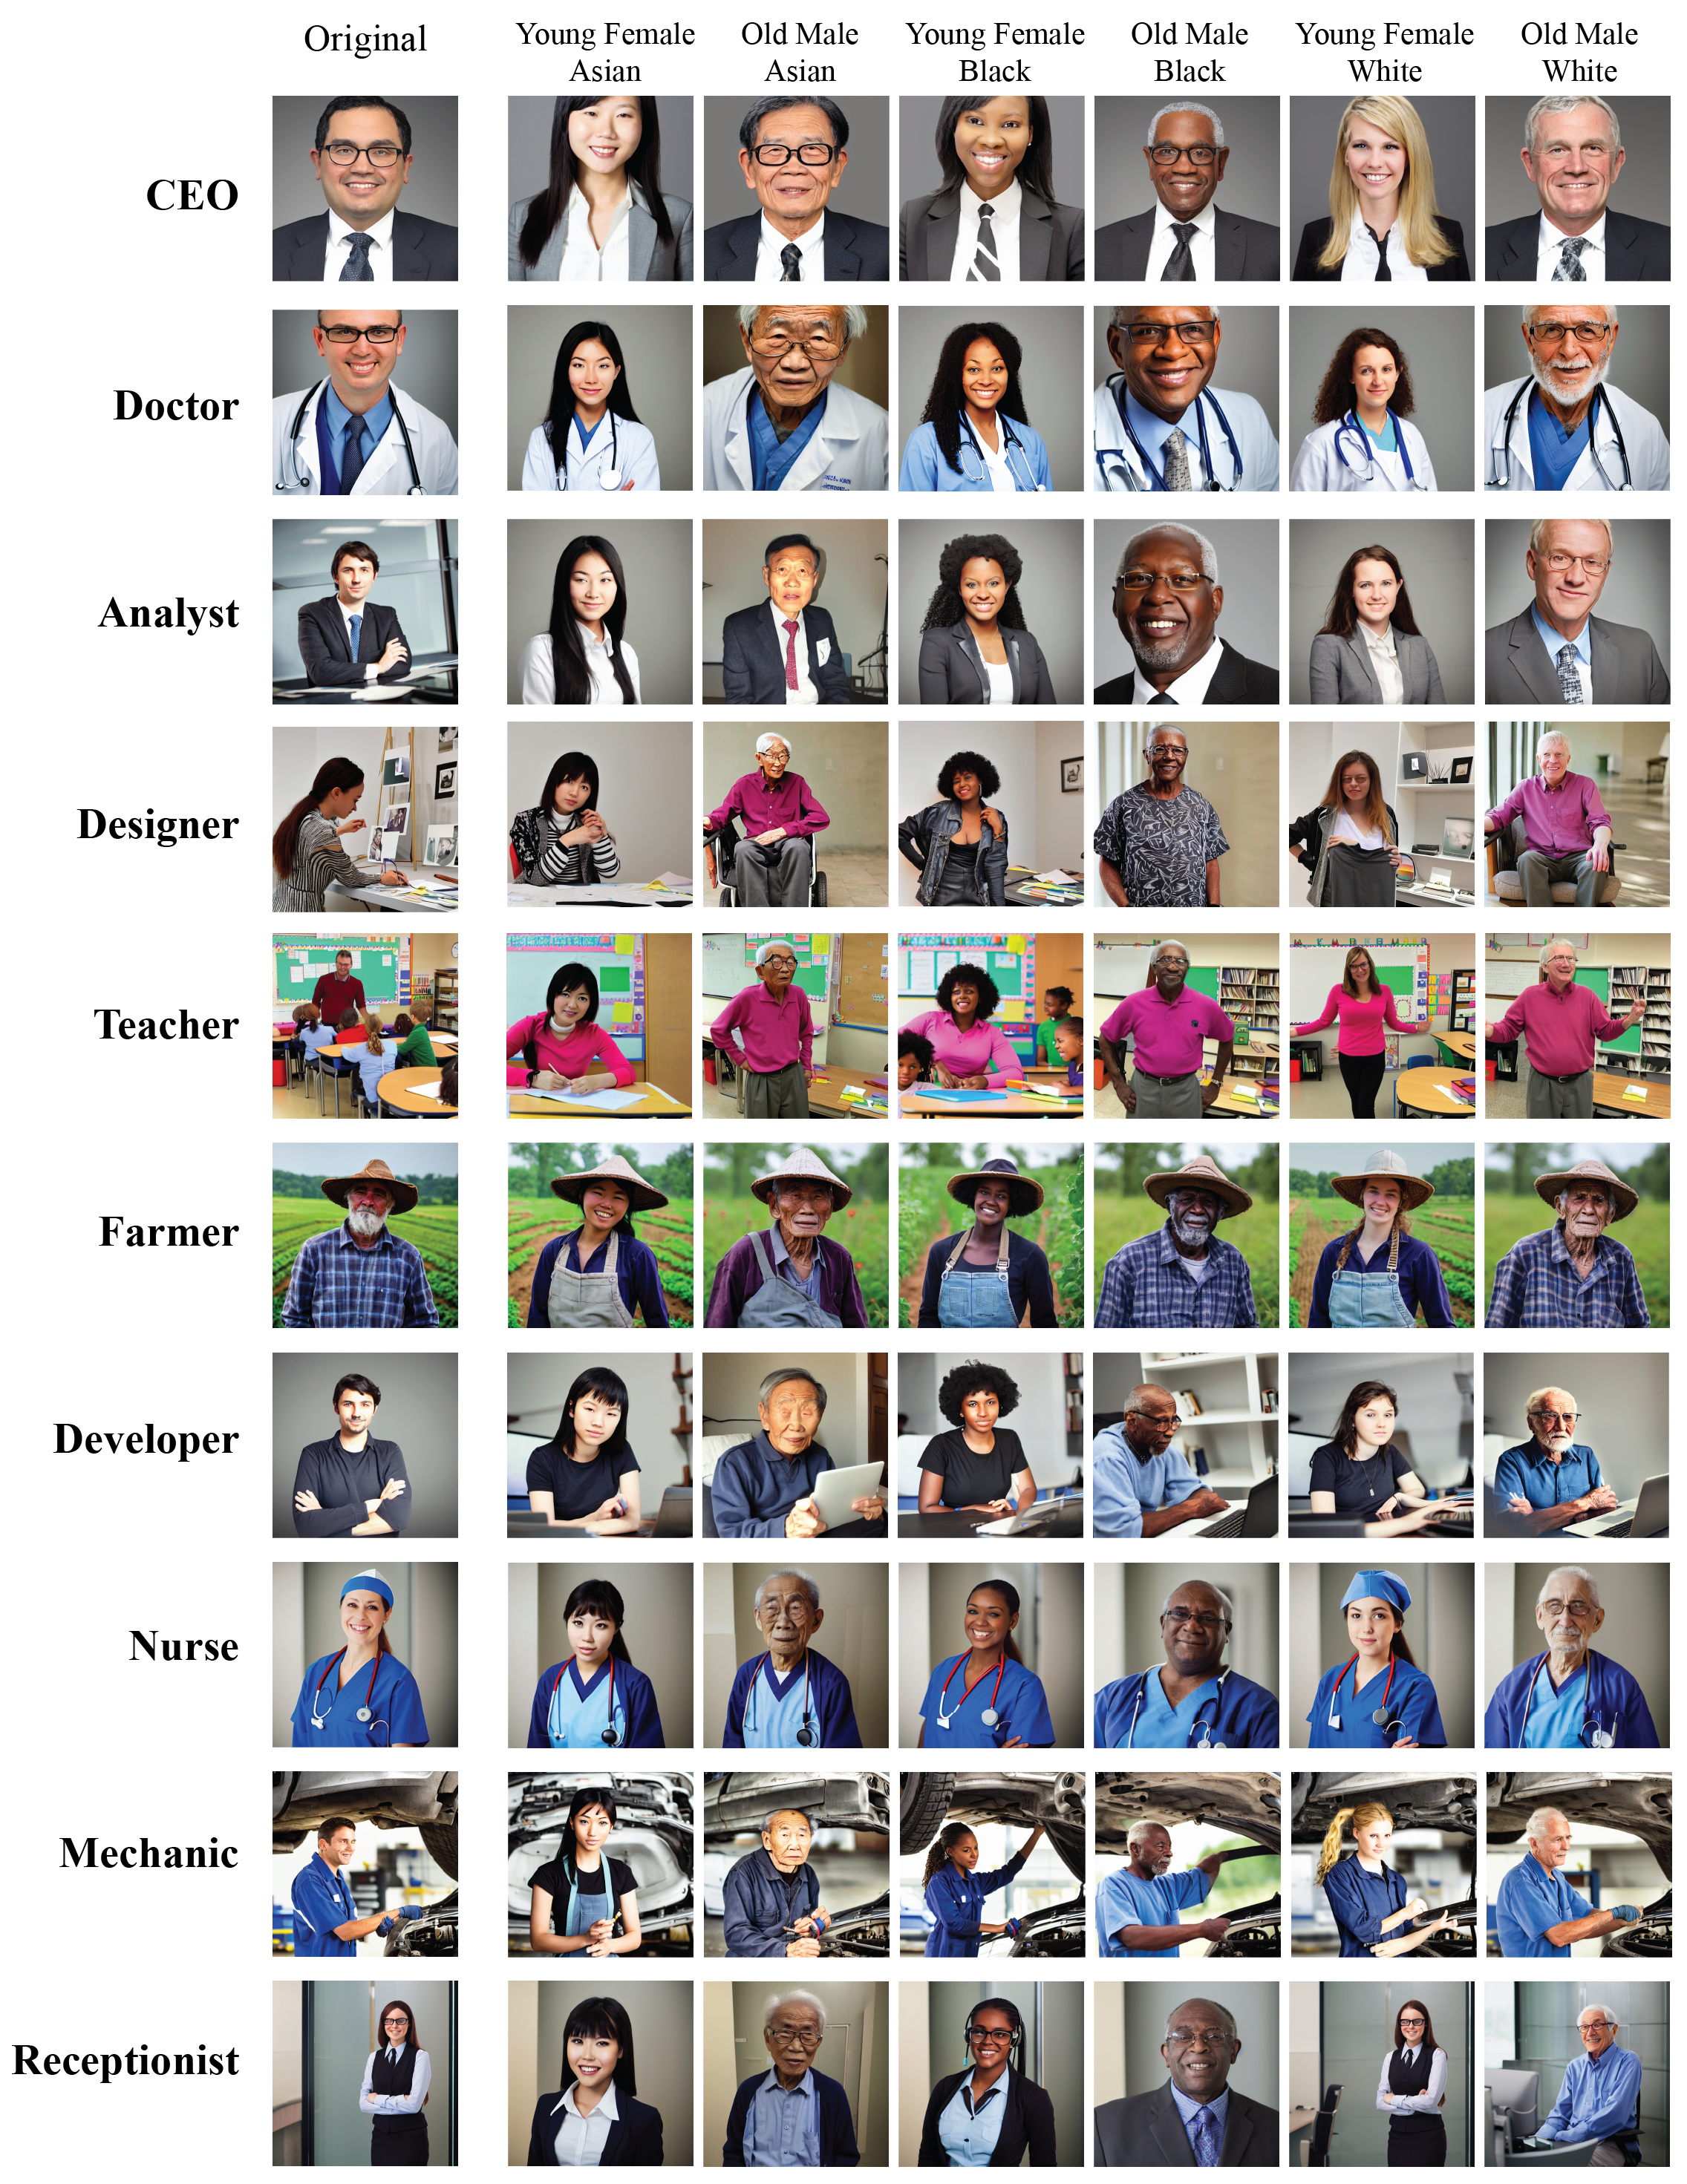}
    \caption{Responsible generation by incorporating multiple aspects simultaneously.
    The figure highlights the ability of the proposed approach to handle composite attributes across professions by leveraging dual-space control. Each row corresponds to a specific profession, with columns showing combination of  attributes for age, gender, and race, incorporated for responsible generation. }
    \label{fig:composite_supp_2}
\end{figure*}

% %%%%%%%%%%%%%%%%%%%
\begin{figure*}
    \centering
    \includegraphics[width=0.9\linewidth]{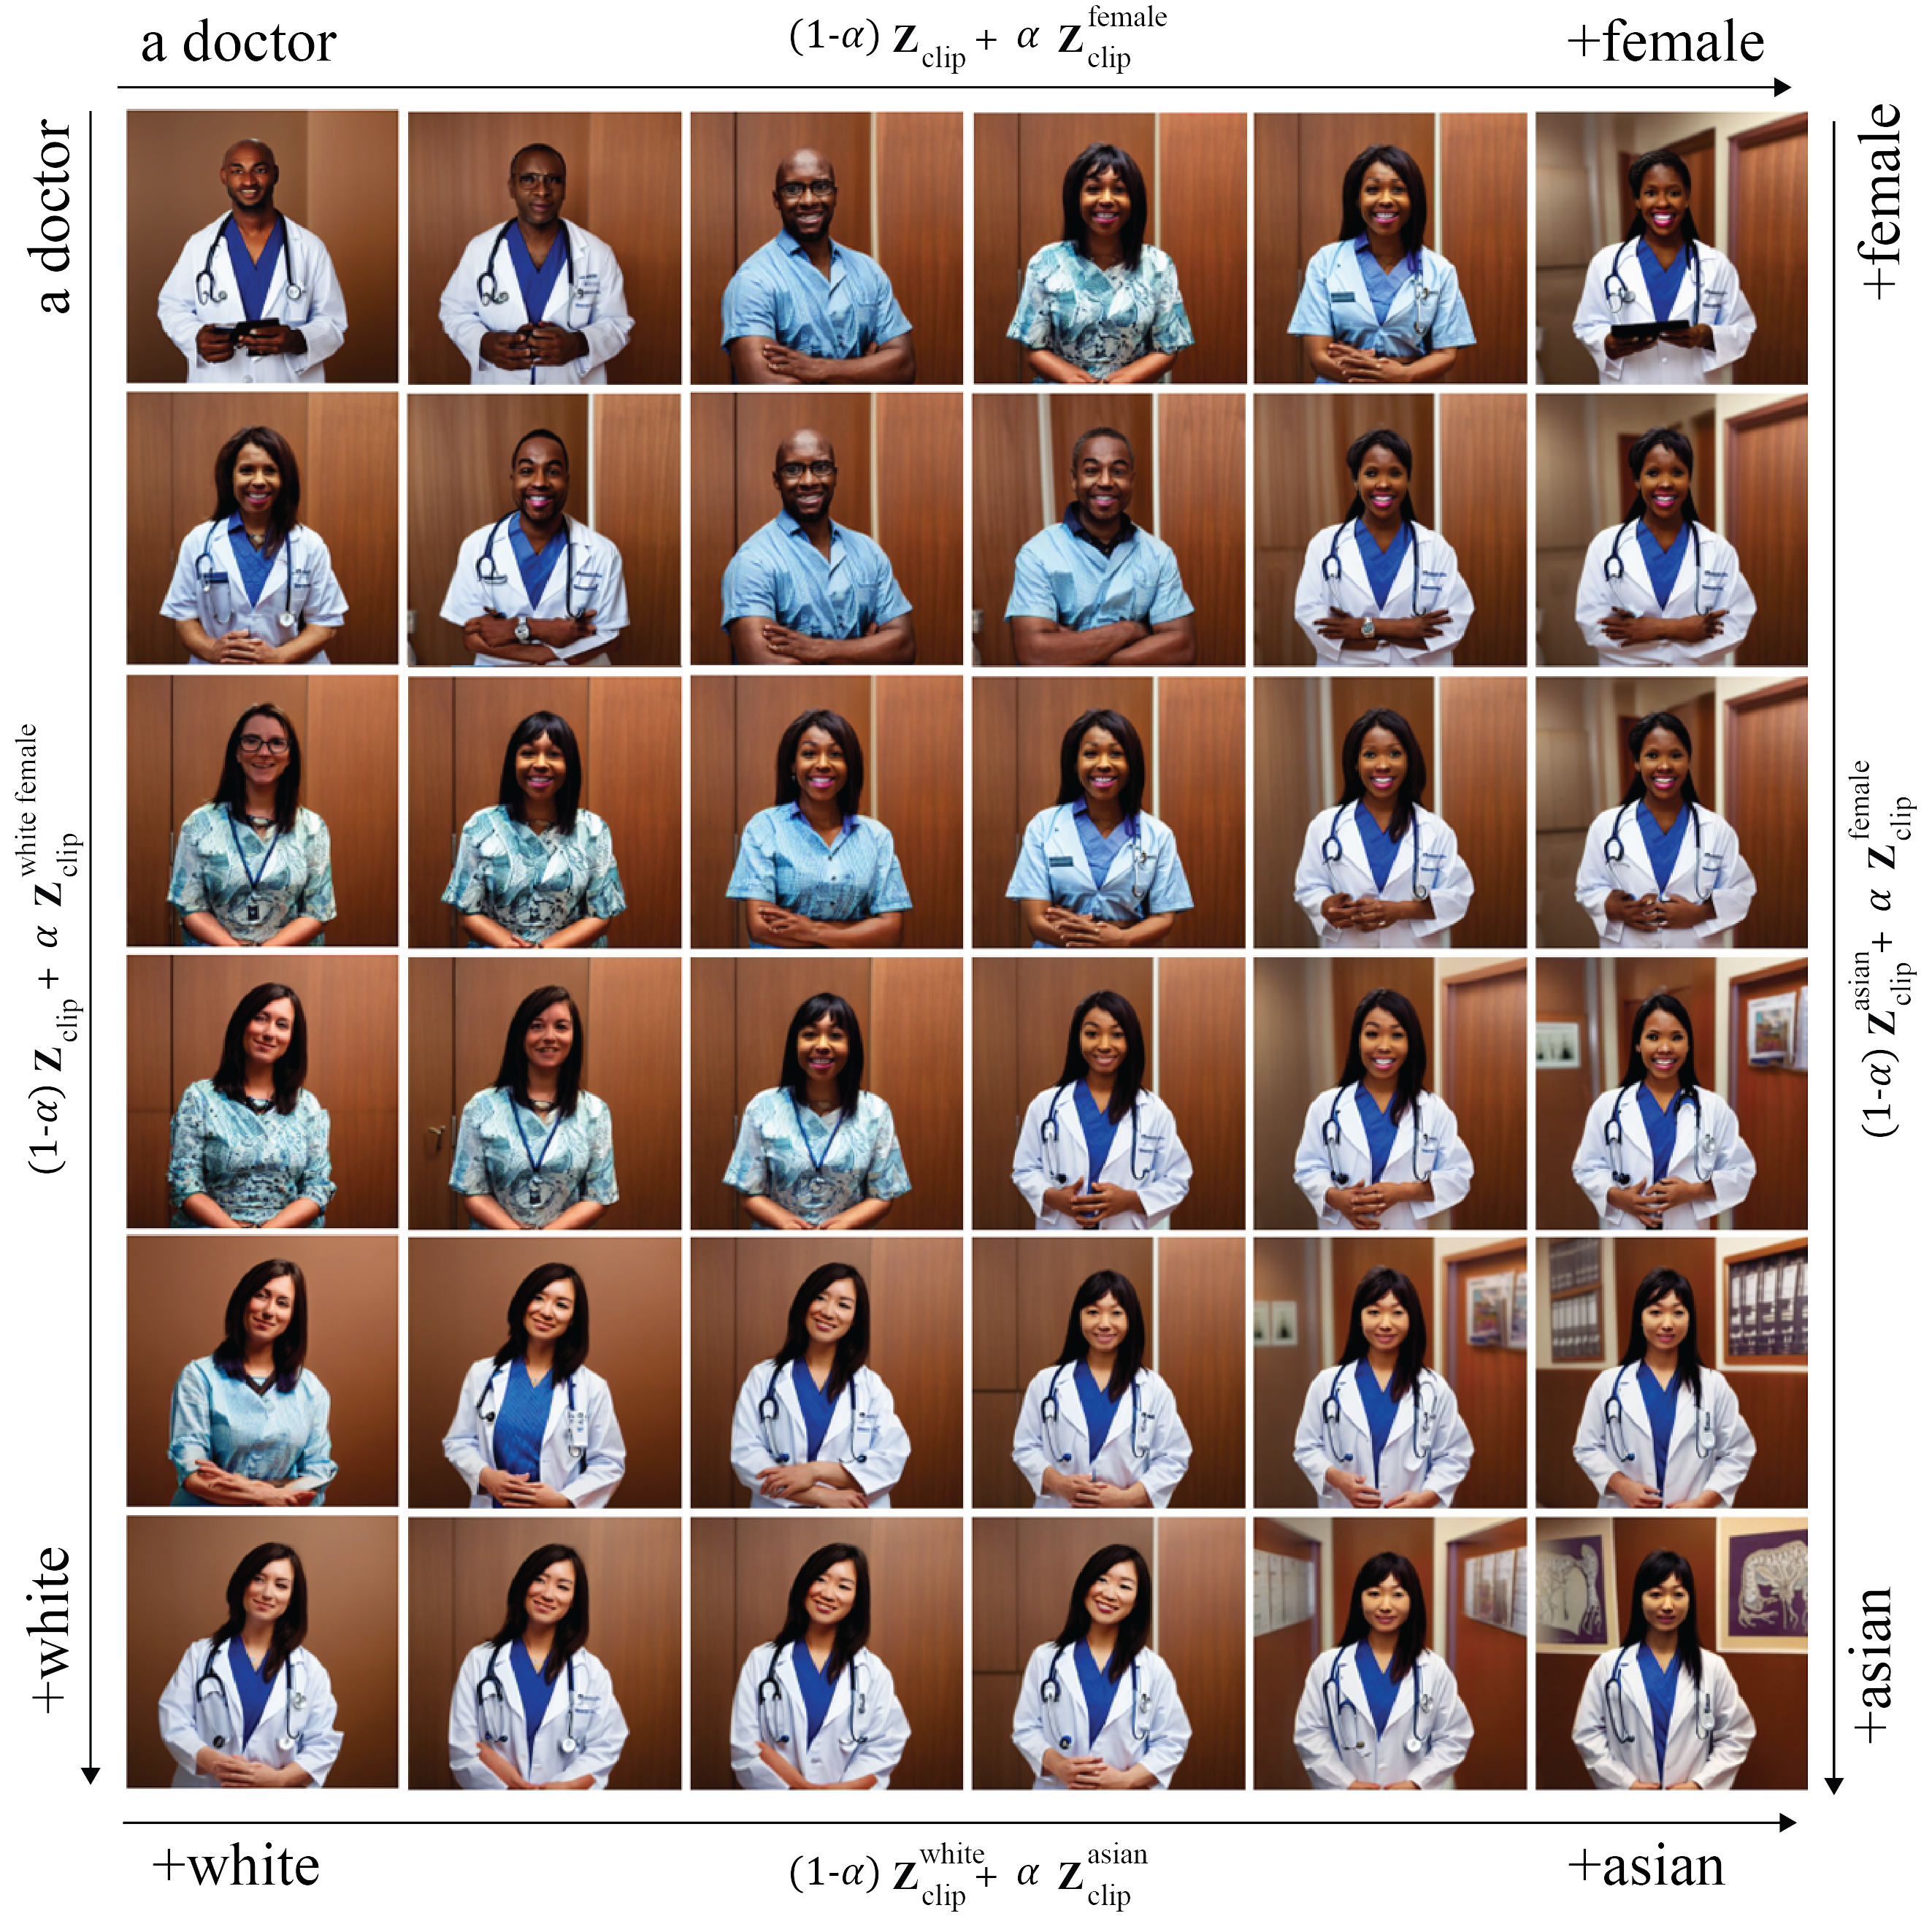}
   \caption{Text embedding space transition caused via RICE. The figure showcases progressive transition by manipulating  $\mathcal{A}_{gender}$ and $\mathcal{A}_{race}$. The corner anchor images represent distinct combinations; images resulting from the interpolated intermediate embeddings present the continuous transition spectrum and showcase the changes as the generated outputs align with the concepts in $\mathcal{A}_{X}$.} 
    \label{fig:embeddings_interpolation}
\end{figure*}

\begin{figure*}
    \centering
    \includegraphics[width=0.9\linewidth]{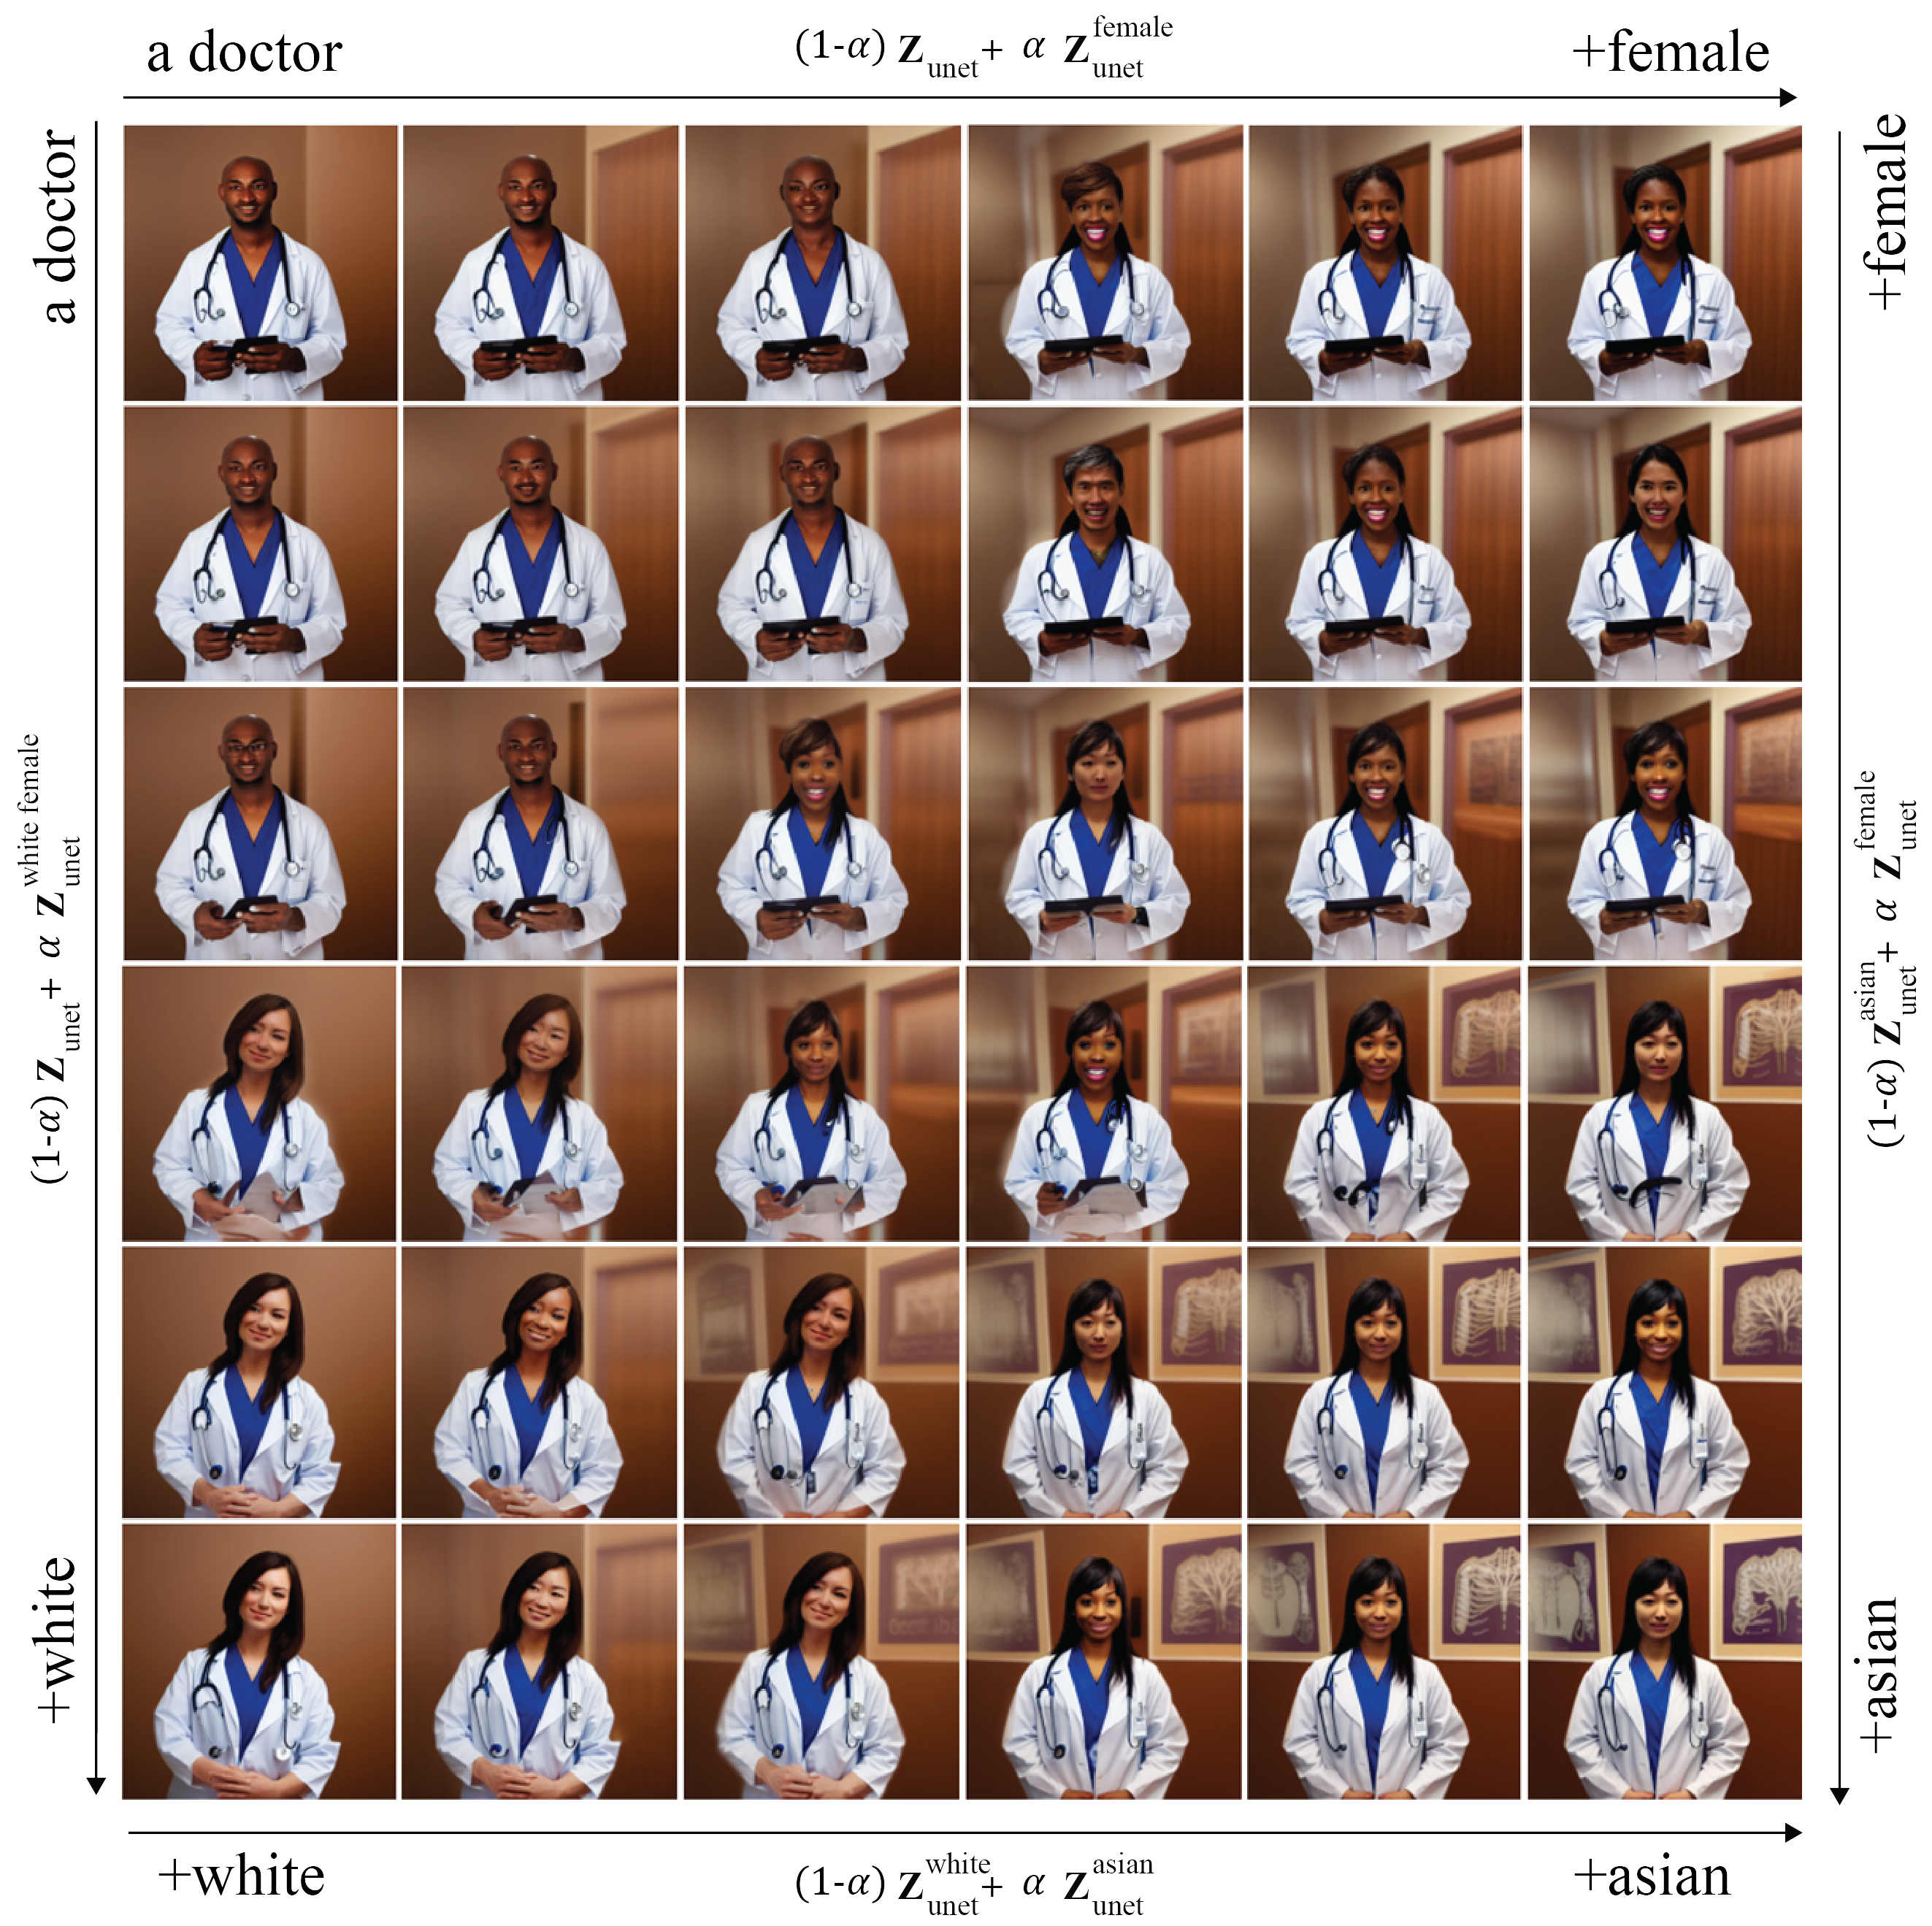}
    \caption{Latent-space refinement caused by RIIDL. The figure showcases RIIDL module  modulating latent diffusion space, progressively aligning outputs with the responsible attributes $\mathcal{A}_{\text{X}}$. Starting from the latent state for <a doctor>, RIIDL enforces control over $\mathcal{A}_{\text{gender}}$ and $\mathcal{A}_{\text{race}}$ by injecting adjustments during denoising. }
    \label{fig:latent_interpolation}
\end{figure*}

\begin{figure*}
\centering
\begin{subfigure}[b]{\textwidth}
   \includegraphics[width=1\linewidth]{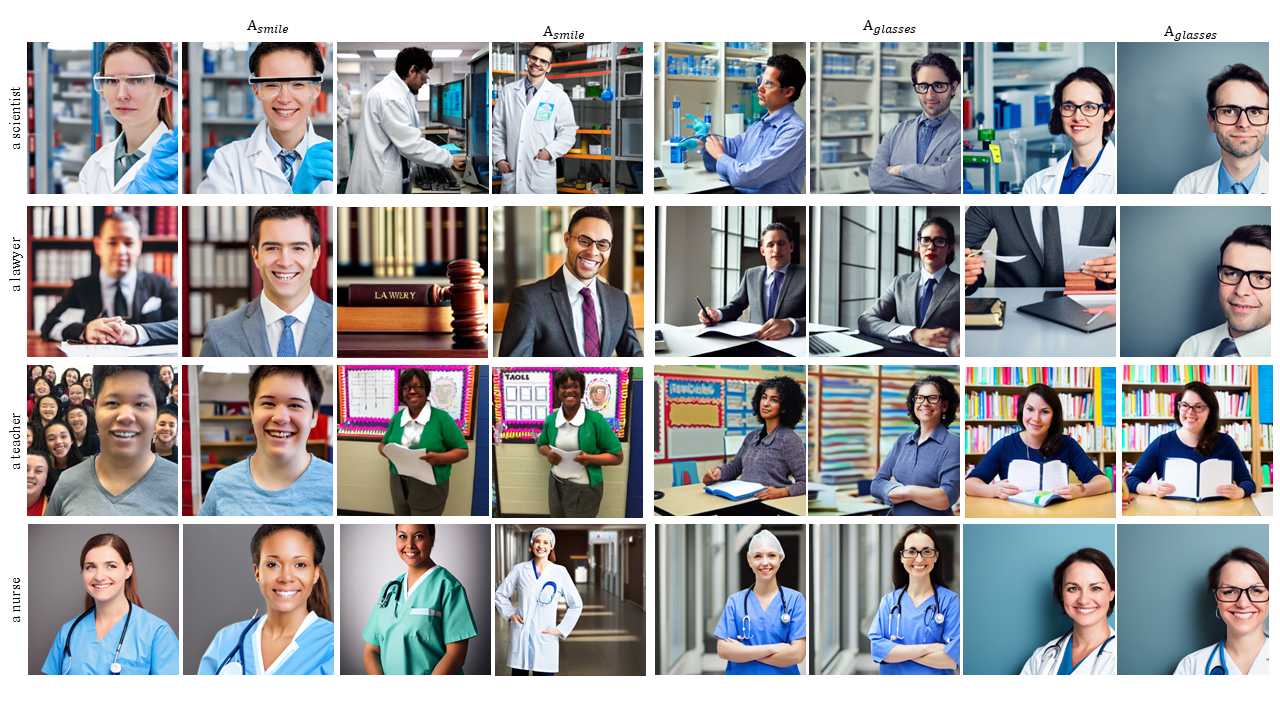}
   \caption{}
   \label{fig:Ng1} 
\end{subfigure}

\begin{subfigure}[b]{\textwidth}
   \includegraphics[width=1\linewidth]{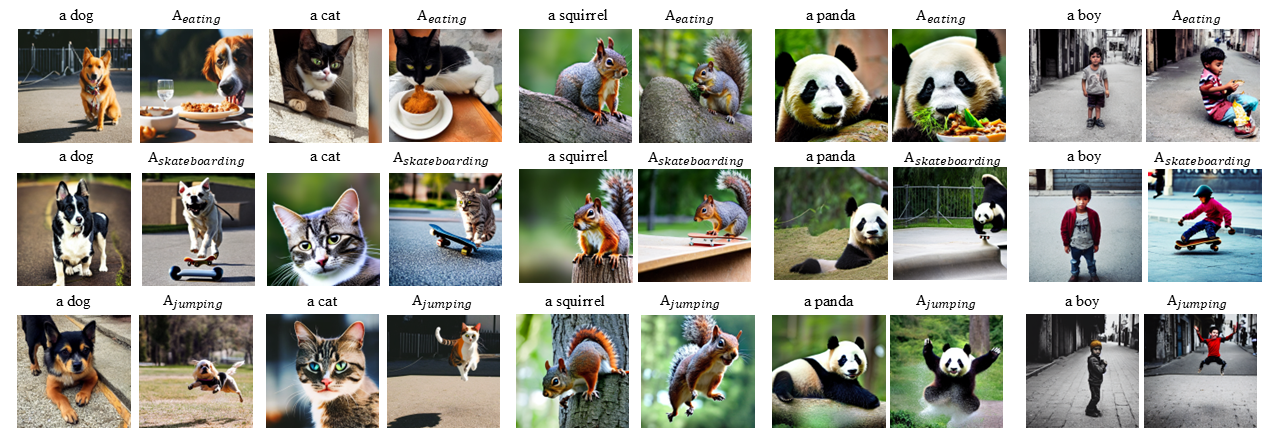}
   \caption{}
   \label{fig:Ng2}
\end{subfigure}

    \caption{Extended attribute control with the proposed method. Additional examples of extending $\mathcal{A}_{\text{X}}$ with attributes beyond core responsible concepts are presented. (a) Shows randomly selected four professions  (scientists, lawyers, teachers, and nurses) for which images are enhanced seamlessly by integrating attributes such as $\mathcal{A}_{\text{smile}}$ and $\mathcal{A}_{\text{glasses}}$ alongside age, gender, and race controls. Notices that the underlying concepts of race, gender and age remain effective besides the additional attributes of smile and glasses. (b) Highlights extensions in a similar manner for animal and object prompts ("a dog," "a cat," "a squirrel", and "a boy") with attributes such as $\mathcal{A}_{\text{eating}}, \mathcal{A}_{\text{skateboarding}}, \mathcal{A}_{\text{jumping}}$, showcasing adaptability and scalability. These results validate the ability of the method to incorporate additional concept spaces while maintaining semantic coherence and visual quality.}

\end{figure*}

\begin{table*}[ht]
    \centering
    \footnotesize % Reduce font size to fit within page width
     \caption{Deviation ratio values across gender and racial attributes in the WinoBias dataset. Lower values indicate better performance. Results for methods: SD, U, and V are also included, where SD: Original Standard Diffusion Model, U: Unified Concept Editing \cite{gandikota2024unified}, V: Vector Interpret Diffusion \cite{li2024self}.}
    \label{tab:supp_fairness}
     % Increase row spacing for readability
    \setlength\tabcolsep{0.1cm} % Adjust column spacing for compactness
    \begin{tabular}{lcccc|cccc|cccc|cccc}
    \toprule
    \multirow{2}{*}{\textbf{Attribute}} & \multicolumn{4}{c}{\cellcolor{gray!15}\textbf{Gender}($\downarrow$)} & \multicolumn{4}{c|}{\cellcolor{gray!15}\textbf{Gender-Pro}($\downarrow$)} & \multicolumn{4}{c}{\cellcolor{gray!15}\textbf{Race}($\downarrow$)} & \multicolumn{4}{c}{\cellcolor{gray!15}\textbf{Race-Pro}($\downarrow$)} \\
    \cmidrule(lr){2-5} \cmidrule(lr){6-9} \cmidrule(lr){10-13} \cmidrule(lr){14-17}
& SD~\cite{Rombach2022} & U~\cite{gandikota2024unified} & V~\cite{li2024self} & Ours & SD~\cite{Rombach2022} & U~\cite{gandikota2024unified} & V~\cite{li2024self} & Ours & SD & U~\cite{gandikota2024unified} & V~\cite{li2024self} & Ours & SD~\cite{Rombach2022} & U~\cite{gandikota2024unified} & V~\cite{li2024self} & Ours \\
    \midrule
    Analyst          & 0.70 & 0.20 & \cellcolor{green!10}0.04 & 0.05 & 0.54 & \cellcolor{green!10}0.04 & 0.08 & 0.08 & 0.82 & 0.29 & 0.24 & \cellcolor{green!10}0.07 & 0.77 & 0.20 & 0.41 & \cellcolor{green!10}0.10 \\
    Assistant        & \cellcolor{green!10}0.02 & 0.14 & 0.37 & 0.04 & 0.48 & 0.80 & 0.45 & \cellcolor{green!10}0.09 & 0.38 & 0.17 & 0.24 & \cellcolor{green!10}0.06 & 0.24 & 0.26 & 0.12 & \cellcolor{green!10}0.08 \\
    Attendant        & 0.16 & 0.09 & 0.24 & \cellcolor{green!10}0.02 & 0.78 & \cellcolor{green!10}0.08 & 0.26 & 0.12 & 0.37 & 0.16 & 0.22 & \cellcolor{green!10}0.07 & 0.67 & 0.37 & 0.13 & \cellcolor{green!10}0.10 \\
    Baker            & 0.82 & 0.29 & \cellcolor{green!10}0.07 & \cellcolor{green!10}0.05 & 0.64 & 1.00 & \cellcolor{green!10}0.09 & 0.11 & 0.83 & 0.14 & 0.12 & \cellcolor{green!10}0.06 & 0.72 & 0.32 & 0.16 & \cellcolor{green!10}0.09 \\
    CEO              & 0.92 & 0.28 & 0.15 & \cellcolor{green!10}0.04 & 0.90 & 0.58 & 0.21 & \cellcolor{green!10}0.13 & 0.38 & 0.13 & 0.22 & \cellcolor{green!10}0.08 & 0.31 & \cellcolor{green!10}0.08 & 0.22 & 0.12 \\
    Carpenter        & 0.92 & 0.06 & \cellcolor{green!10}0.02 & 0.06 & 1.00 & 1.00 & \cellcolor{green!10}0.03 & 0.14 & 0.91 & 0.12 & 0.28 & \cellcolor{green!10}0.08 & 0.83 & 0.65 & 0.26 & \cellcolor{green!10}0.11 \\

    Cashier          & 0.74 & 0.16 & 0.63 & \cellcolor{green!10}0.03 & 0.92 & 0.92 & 0.66 & \cellcolor{green!10}0.15 & 0.45 & 0.43 & 0.34 & \cellcolor{green!10}0.07 & 0.46 & 0.41 & 0.30 & \cellcolor{green!10}0.09 \\
    Cleaner          & 0.54 & 0.33 & \cellcolor{green!10}0.06 & \cellcolor{green!10}0.04 & 0.30 & 0.80 & \cellcolor{green!10}0.08 & \cellcolor{green!10}0.09 & \cellcolor{green!10}0.10 & 0.28 & 0.14 & \cellcolor{green!10}0.06 & 0.45 & 0.55 & 0.26 & \cellcolor{green!10}0.08 \\
    Clerk            & 0.14 & 0.23 & 0.42 & \cellcolor{green!10}0.04 & 0.58 & 0.96 & 0.46 & \cellcolor{green!10}0.12 & 0.46 & 0.25 & 0.16 & \cellcolor{green!10}0.07 & 0.59 & 0.38 & 0.16 & \cellcolor{green!10}0.10 \\
    Const. Worker    & 1.00 & \cellcolor{green!10}0.06 & 0.80 & \cellcolor{green!10}0.05 & 1.00 & 0.24 & 0.84 & \cellcolor{green!10}0.11 & 0.41 & 0.16 & 0.26 & \cellcolor{green!10}0.08 & 0.44 & 0.29 & 0.25 & \cellcolor{green!10}0.12 \\
    Cook             & 0.72 & \cellcolor{green!10}0.03 & \cellcolor{green!10}0.04 & 0.05 & \cellcolor{green!10}0.02 & 0.36 & 0.07 & \cellcolor{green!10}0.08 & 0.56 & 0.15 & 0.30 & \cellcolor{green!10}0.07 & 0.18 & 0.49 & 0.14 & 0.10 \\
    Counselor        & \cellcolor{green!10}0.00 & 0.40 & 0.45 & \cellcolor{green!10}0.04 & 0.56 & 1.00 & 0.47 & \cellcolor{green!10}0.16 & 0.72 & 0.19 & 0.16 & \cellcolor{green!10}0.07 & 0.36 & 0.79 & 0.12 & \cellcolor{green!10}0.09 \\
    Designer         & 0.12 & \cellcolor{green!10}0.07 & 0.28 & \cellcolor{green!10}0.03 & 0.72 & 0.84 & 0.30 & \cellcolor{green!10}0.10 & 0.14 & 0.23 & \cellcolor{green!10}0.10 & \cellcolor{green!10}0.06 & 0.18 & 0.34 & 0.15 & \cellcolor{green!10}0.11 \\
    Developer        & 0.90 & 0.51 & 0.54 & \cellcolor{green!10}0.04 & 0.92 & 0.96 & 0.58 & \cellcolor{green!10}0.14 & 0.41 & 0.23 & 0.30 & \cellcolor{green!10}0.08 & 0.32 & 0.20 & 0.39 & \cellcolor{green!10}0.13 \\
    Doctor           & 0.92 & 0.20 & \cellcolor{green!10}0.08 & 0.05 & 0.52 & 0.32 & \cellcolor{green!10}0.10 & \cellcolor{green!10}0.10 & 0.92 & \cellcolor{green!10}0.07 & 0.26 & \cellcolor{green!10}0.07 & 0.59 & 0.52 & 0.15 & \cellcolor{green!10}0.12 \\
    Driver           & 0.90 & 0.21 & 0.12 & \cellcolor{green!10}0.04 & 0.48 & 0.60 & 0.14 & \cellcolor{green!10}0.09 & 0.34 & 0.23 & 0.16 & \cellcolor{green!10}0.08 & 0.25 & 0.26 & \cellcolor{green!10}0.07 & 0.10 \\
    Farmer           & 1.00 & 0.41 & 0.21 & \cellcolor{green!10}0.03 & 0.98 & \cellcolor{green!10}0.12 & 0.30 & \cellcolor{green!10}0.08 & 0.95 & 0.27 & 0.50 & \cellcolor{green!10}0.07 & 0.39 & 0.82 & 0.28 & \cellcolor{green!10}0.09 \\
    
        Guard            & 0.78 & 0.12 & 0.14 & \cellcolor{green!10}0.04 & 0.76 & \cellcolor{green!10}0.08 & 0.17 & 0.15 & 0.20 & 0.16 & \cellcolor{green!10}0.12 & \cellcolor{green!10}0.09 & 0.35 & 0.23 & 0.14 & \cellcolor{green!10}0.10 \\
    Hairdresser      & 0.92 & 0.16 & 0.84 & \cellcolor{green!10}0.05 & 0.88 & 0.46 & 0.86 & \cellcolor{green!10}0.17 & 0.45 & 0.31 & 0.42 & \cellcolor{green!10}0.07 & 0.38 & \cellcolor{green!10}0.05 & 0.23 & 0.12 \\
    Housekeeper      & 0.96 & 0.41 & 0.90 & \cellcolor{green!10}0.04 & 1.00 & 1.00 & 0.91 & \cellcolor{green!10}0.13 & 0.45 & \cellcolor{green!10}0.07 & 0.28 & \cellcolor{green!10}0.07 & 0.45 & 0.41 & 0.34 & \cellcolor{green!10}0.09 \\
    Janitor          & 0.96 & 0.16 & 0.44 & \cellcolor{green!10}0.05 & 0.94 & \cellcolor{green!10}0.08 & 0.46 & \cellcolor{green!10}0.14 & 0.35 & \cellcolor{green!10}0.14 & 0.24 & \cellcolor{green!10}0.06 & 0.40 & 0.24 & \cellcolor{green!10}0.07 & \cellcolor{green!10}0.10 \\
    Laborer          & 1.00 & \cellcolor{green!10}0.09 & 0.41 & \cellcolor{green!10}0.05 & 0.98 & \cellcolor{green!10}0.08 & 0.43 & \cellcolor{green!10}0.08 & 0.33 & 0.40 & 0.24 & \cellcolor{green!10}0.10 & 0.53 & 0.38 & 0.20 & \cellcolor{green!10}0.11 \\
    Lawyer           & 0.68 & 0.30 & \cellcolor{green!10}0.10 & \cellcolor{green!10}0.04 & 0.36 & 0.18 & 0.17 & \cellcolor{green!10}0.12 & 0.64 & 0.20 & 0.18 & \cellcolor{green!10}0.08 & 0.52 & \cellcolor{green!10}0.14 & 0.13 & \cellcolor{green!10}0.09 \\
    Librarian        & 0.66 & \cellcolor{green!10}0.07 & 0.81 & \cellcolor{green!10}0.03 & 0.54 & 0.40 & 0.86 & \cellcolor{green!10}0.09 & 0.85 & 0.28 & 0.42 & \cellcolor{green!10}0.06 & 0.74 & 0.16 & 0.27 & \cellcolor{green!10}0.10 \\
    Manager          & 0.46 & 0.19 & \cellcolor{green!10}0.10 & \cellcolor{green!10}0.05 & 0.62 & 0.40 & 0.91 & \cellcolor{green!10}0.10 & 0.69 & 0.17 & 0.24 & \cellcolor{green!10}0.08 & 0.41 & 0.17 & 0.19 & \cellcolor{green!10}0.12 \\
    Mechanic         & 1.00 & 0.23 & 0.34 & \cellcolor{green!10}0.04 & 0.98 & 0.48 & 0.46 & \cellcolor{green!10}0.11 & 0.64 & 0.22 & 0.14 & \cellcolor{green!10}0.07 & 0.47 & 0.44 & \cellcolor{green!10}0.05 & \cellcolor{green!10}0.08 \\
    Nurse            & 1.00 & 0.39 & 0.96 & \cellcolor{green!10}0.04 & 0.98 & 0.84 & 0.43 & \cellcolor{green!10}0.18 & 0.76 & 0.25 & 0.30 & \cellcolor{green!10}0.07 & 0.39 & 0.79 & \cellcolor{green!10}0.08 & 0.14 \\
    Physician        & 0.78 & 0.42 & \cellcolor{green!10}0.06 & 0.05 & 0.30 & 0.16 & 0.17 & \cellcolor{green!10}0.08 & 0.67 & \cellcolor{green!10}0.08 & 0.18 & \cellcolor{green!10}0.08 & 0.46 & 0.58 & \cellcolor{green!10}0.02 & \cellcolor{green!10}0.10 \\
    Receptionist     & 0.84 & 0.38 & 0.88 & \cellcolor{green!10}0.04 & 0.98 & 0.96 & 0.86 & \cellcolor{green!10}0.17 & 0.88 & \cellcolor{green!10}0.10 & 0.36 & \cellcolor{green!10}0.07 & 0.74 & \cellcolor{green!10}0.14 & 0.25 & \cellcolor{green!10}0.11 \\
    Salesperson      & 0.68 & 0.38 & \cellcolor{green!10}0.04 & \cellcolor{green!10}0.04 & 0.54 & \cellcolor{green!10}0.12 & 0.18 & \cellcolor{green!10}0.11 & 0.69 & 0.32 & 0.26 & \cellcolor{green!10}0.07 & 0.66 & 0.19 & 0.36 & \cellcolor{green!10}0.13 \\
    Secretary        & 0.64 & \cellcolor{green!10}0.10 & 0.76 & \cellcolor{green!10}0.04 & 0.92 & 0.96 & 0.44 & \cellcolor{green!10}0.14 & 0.37 & 0.35 & 0.24 & \cellcolor{green!10}0.06 & 0.55 & 0.43 & 0.32 & \cellcolor{green!10}0.09 \\
    Sheriff          & 1.00 & \cellcolor{green!10}0.10 & 0.24 & \cellcolor{green!10}0.05 & 0.98 & \cellcolor{green!10}0.24 & 0.97 & \cellcolor{green!10}0.12 & 0.82 & 0.17 & 0.18 & \cellcolor{green!10}0.08 & 0.74 & 0.35 & 0.27 & \cellcolor{green!10}0.10 \\
    Supervisor       & 0.64 & 0.26 & 0.16 & \cellcolor{green!10}0.05 & 0.52 & 0.46 & \cellcolor{green!10}0.12 & \cellcolor{green!10}0.10 & 0.49 & 0.14 & 0.14 & \cellcolor{green!10}0.07 & 0.45 & 0.31 & 0.14 & 0.12 \\
    Tailor           & 0.56 & 0.27 & 0.14 & \cellcolor{green!10}0.04 & 0.78 & 0.48 & 0.89 & \cellcolor{green!10}0.08 & 0.16 & 0.20 & \cellcolor{green!10}0.10 & \cellcolor{green!10}0.07 & \cellcolor{green!10}0.14 & 0.19 & 0.13 & \cellcolor{green!10}0.09 \\
    Teacher          & 0.30 & \cellcolor{green!10}0.06 & 0.51 & \cellcolor{green!10}0.04 & 0.48 & 0.16 & \cellcolor{green!10}0.07 & 0.13 & 0.51 & 0.10 & \cellcolor{green!10}0.04 & 0.08 & 0.26 & 0.23 & 0.21 & \cellcolor{green!10}0.10 \\
    Writer           & \cellcolor{green!10}0.04 & 0.31 & 0.49 & \cellcolor{green!10}0.04 & 0.26 & 0.52 & 0.91 & \cellcolor{green!10}0.10 & 0.86 & 0.23 & 0.26 & \cellcolor{green!10}0.06 & 0.69 & 0.38 & \cellcolor{green!10}0.07 & \cellcolor{green!10}0.09 \\ \hline
    Average         & 0.68 & 0.22 & 0.36 & \cellcolor{green!10}0.04 & 0.70 & 0.52 & 0.61 & \cellcolor{green!10}0.14 & 0.56 & 0.21 & 0.23 & \cellcolor{green!10}0.07 & 0.48 & 0.35 & 0.20 & \cellcolor{green!10}0.10 \\
    
    \bottomrule
    \end{tabular}
   
\end{table*}

\begin{table*}
    \centering
    \small
    \caption{Debaising performance across professions in Winobias dataset \cite{zhao2018gender}. The metric $\Delta = 0$ indicate ideal debaising. Our method shows very strong performance compared to previous approaches.}
        \label{tab:merged_debiasing_performance}

    \begin{tabular}{lcccccc}
        \toprule
        \cellcolor{gray!15}\textbf{Profession} & \cellcolor{gray!15}\textbf{SD} & \cellcolor{gray!15}\textbf{ CA}~\cite{wang2023concept} &\cellcolor{gray!15} \textbf{DVL}~\cite{chuang2023debiasing} & \cellcolor{gray!15}\textbf{TIME}~\cite{orgad2023editing} & \cellcolor{gray!15}\textbf{TIMEP}~\cite{gandikota2024unified} & \cellcolor{gray!15}\textbf{Ours} \\ 
        \midrule
        Attendant      & \cellcolor{green!10}0.13 $\pm$ 0.06 & 0.23 $\pm$ 0.08 & 0.30 $\pm$ 0.04 & 0.50 $\pm$ 0.01 & 0.38 $\pm$ 0.11 & \cellcolor{green!10}0.09 $\pm$ 0.04 \\
        Cashier        & 0.67 $\pm$ 0.04 & 0.71 $\pm$ 0.10 & \cellcolor{green!10}0.23 $\pm$ 0.07 & 0.46 $\pm$ 0.01 & 0.23 $\pm$ 0.15 & \cellcolor{green!10}0.16 $\pm$ 0.06 \\
        Teacher        & 0.42 $\pm$ 0.01 & 0.46 $\pm$ 0.00 & 0.11 $\pm$ 0.05 & 0.34 $\pm$ 0.06 & \cellcolor{green!10}0.07 $\pm$ 0.06 &\cellcolor{green!10} 0.05 $\pm$ 0.01 \\
        Nurse          & 0.99 $\pm$ 0.01 & 0.91 $\pm$ 0.05 & 0.87 $\pm$ 0.01 & 0.34 $\pm$ 0.03 & \cellcolor{green!10} 0.20 $\pm$ 0.09 &\cellcolor{green!10}  0.20 $\pm$ 0.07 \\
        Assistant      & 0.19 $\pm$ 0.05 & 0.20 $\pm$ 0.07 & 0.35 $\pm$ 0.15 & 0.32 $\pm$ 0.06 & 0.57 $\pm$ 0.08 & \cellcolor{green!10} 0.14 $\pm$ 0.06 \\
        Secretary      & 0.88 $\pm$ 0.01 & 0.65 $\pm$ 0.07 & 0.65 $\pm$ 0.01 & 0.58 $\pm$ 0.09 & 0.71 $\pm$ 0.02 & \cellcolor{green!10}0.10 $\pm$ 0.10 \\
        Cleaner        & 0.38 $\pm$ 0.04 &\cellcolor{green!10} 0.11 $\pm$ 0.06 & 0.18 $\pm$ 0.04 & 0.58 $\pm$ 0.07 & 0.79 $\pm$ 0.04 & \cellcolor{green!10}0.13 $\pm$ 0.07 \\
        Receptionist   & 0.99 $\pm$ 0.01 & 0.90 $\pm$ 0.08 & 0.74 $\pm$ 0.04 & 0.36 $\pm$ 0.10 & 0.24 $\pm$ 0.12 &\cellcolor{green!10} 0.10 $\pm$ 0.01 \\
        Clerk          & 0.10 $\pm$ 0.07 & \cellcolor{green!10}0.11 $\pm$ 0.08 & 0.10 $\pm$ 0.04 & 0.40 $\pm$ 0.03 & 0.76 $\pm$ 0.05 &\cellcolor{green!10} 0.23 $\pm$ 0.06 \\
        Counselor      & \cellcolor{green!10}0.06 $\pm$ 0.05 & 0.30 $\pm$ 0.03 & 0.10 $\pm$ 0.07 & 0.74 $\pm$ 0.08 & 0.41 $\pm$ 0.06 &0.11 $\pm$ 0.02 \\
        Designer       & 0.23 $\pm$ 0.05 & 0.25 $\pm$ 0.12 & 0.48 $\pm$ 0.06 & 0.44 $\pm$ 0.06 & 0.23 $\pm$ 0.16 & \cellcolor{green!10}0.07 $\pm$ 0.05 \\
        Hairdresser    & 0.74 $\pm$ 0.11 & 0.37 $\pm$ 0.16 & 0.61 $\pm$ 0.04 & 0.32 $\pm$ 0.01 & 0.41 $\pm$ 0.09 & \cellcolor{green!10}0.10 $\pm$ 0.04 \\
        Writer         & 0.15 $\pm$ 0.03 & 0.07 $\pm$ 0.03 & 0.45 $\pm$ 0.04 & 0.54 $\pm$ 0.08 & 0.52 $\pm$ 0.08 &\cellcolor{green!10} 0.09 $\pm$ 0.08 \\
        Housekeeper    & 0.93 $\pm$ 0.04 & 0.68 $\pm$ 0.18 & 0.80 $\pm$ 0.07 & 0.32 $\pm$ 0.03 & 0.68 $\pm$ 0.07 & \cellcolor{green!10}0.08 $\pm$ 0.05 \\
        Baker          & 0.81 $\pm$ 0.01 & \cellcolor{green!10}0.19 $\pm$ 0.04 & 0.72 $\pm$ 0.05 & 0.40 $\pm$ 0.04 & \cellcolor{green!10}0.19 $\pm$ 0.14 & 0.20 $\pm$ 0.08 \\
        Librarian      & 0.86 $\pm$ 0.06 & 0.66 $\pm$ 0.07 & 0.34 $\pm$ 0.06 & 0.26 $\pm$ 0.05 & 0.35 $\pm$ 0.01 & \cellcolor{green!10}0.04 $\pm$ 0.02 \\
        Tailor         & 0.30 $\pm$ 0.01 & 0.21 $\pm$ 0.05 & 0.33 $\pm$ 0.11 & 0.50 $\pm$ 0.03 &\cellcolor{green!10} 0.03 $\pm$ 0.00 & 0.20 $\pm$ 0.01 \\
        Driver         & 0.97 $\pm$ 0.02 & 0.20 $\pm$ 0.07 & 0.65 $\pm$ 0.04 & 0.48 $\pm$ 0.09 & \cellcolor{green!10}0.11 $\pm$ 0.08 & 0.21 $\pm$ 0.07 \\
        Supervisor     & 0.50 $\pm$ 0.01 & 0.07 $\pm$ 0.03 & 0.43 $\pm$ 0.04 & 0.50 $\pm$ 0.07 & 0.42 $\pm$ 0.03 & \cellcolor{green!10}0.26 $\pm$ 0.04 \\
        Janitor        & 0.91 $\pm$ 0.05 & 0.71 $\pm$ 0.06 & 0.75 $\pm$ 0.05 & 0.36 $\pm$ 0.08 & 0.47 $\pm$ 0.12 & \cellcolor{green!10} 0.16 $\pm$ 0.04 \\
        Cook           & 0.82 $\pm$ 0.04 & 0.48 $\pm$ 0.16 & 0.52 $\pm$ 0.07 & 0.38 $\pm$ 0.03 & 0.15 $\pm$ 0.10 & \cellcolor{green!10}0.03 $\pm$ 0.02 \\
        Laborer        & 0.99 $\pm$ 0.01 & 0.81 $\pm$ 0.06 & 0.98 $\pm$ 0.03 & 0.48 $\pm$ 0.08 & 0.24 $\pm$ 0.09 & \cellcolor{green!10}0.09 $\pm$ 0.02 \\
        Constr. worker & 1.00 $\pm$ 0.00 & 0.95 $\pm$ 0.01 & 1.00 $\pm$ 0.00 & 0.40 $\pm$ 0.01 & 0.15 $\pm$ 0.05 & \cellcolor{green!10}0.06 $\pm$ 0.04 \\
        Developer      & 0.90 $\pm$ 0.03 & 0.74 $\pm$ 0.02 & 0.90 $\pm$ 0.04 & 0.50 $\pm$ 0.01 & 0.47 $\pm$ 0.07 & \cellcolor{green!10}0.08 $\pm$ 0.02 \\
        Carpenter      & 0.92 $\pm$ 0.05 & 0.84 $\pm$ 0.01 & 0.98 $\pm$ 0.01 & 0.52 $\pm$ 0.06 & 0.52 $\pm$ 0.05 & \cellcolor{green!10}0.06 $\pm$ 0.02 \\
        Manager        & 0.54 $\pm$ 0.06 &\cellcolor{green!10} 0.15 $\pm$ 0.01 & 0.30 $\pm$ 0.05 & 0.38 $\pm$ 0.05 &\cellcolor{green!10} 0.10 $\pm$ 0.01 & 0.19 $\pm$ 0.07 \\
        Lawyer         & 0.46 $\pm$ 0.08 &\cellcolor{green!10} 0.13 $\pm$ 0.06 & 0.52 $\pm$ 0.05 & 0.64 $\pm$ 0.03 & 0.15 $\pm$ 0.03 & 0.30 $\pm$ 0.07 \\
        Farmer         & 0.97 $\pm$ 0.02 & 0.58 $\pm$ 0.09 & 0.97 $\pm$ 0.02 & 0.46 $\pm$ 0.02 & 0.27 $\pm$ 0.08 & \cellcolor{green!10}0.09 $\pm$ 0.01 \\
        Salesperson    & 0.60 $\pm$ 0.08 & 0.18 $\pm$\cellcolor{green!10} 0.05 & 0.07 $\pm$ 0.05 & 0.52 $\pm$ 0.05 &\cellcolor{green!10} 0.05 $\pm$ 0.01 & 0.11 $\pm$ 0.05 \\
        Physician      & 0.62 $\pm$ 0.14 & 0.36 $\pm$ 0.10 & 0.70 $\pm$ 0.07 & 0.56 $\pm$ 0.06 & 0.49 $\pm$ 0.04 & \cellcolor{green!10}0.11 $\pm$ 0.04 \\
        Guard          & 0.86 $\pm$ 0.02 & 0.43 $\pm$ 0.12 & 0.48 $\pm$ 0.06 & 0.30 $\pm$ 0.10 &\cellcolor{green!10} 0.10 $\pm$ 0.12 & \cellcolor{green!10}0.12 $\pm$ 0.07 \\
        Analyst        & 0.58 $\pm$ 0.12 & 0.24 $\pm$ 0.18 & 0.71 $\pm$ 0.02 & 0.52 $\pm$ 0.03 & 0.13 $\pm$ 0.05 & \cellcolor{green!10}0.07 $\pm$ 0.02 \\
        Mechanic       & 0.99 $\pm$ 0.01 & 0.65 $\pm$ 0.04 & 0.92 $\pm$ 0.01 & 0.38 $\pm$ 0.09 & 0.21 $\pm$ 0.04 & \cellcolor{green!10}0.13 $\pm$ 0.08 \\
        Sheriff        & 0.99 $\pm$ 0.01 & 0.38 $\pm$ 0.22 & 0.82 $\pm$ 0.08 & 0.22 $\pm$ 0.05 & 0.10 $\pm$ 0.05 & \cellcolor{green!10}0.06 $\pm$ 0.03 \\
        CEO            & 0.87 $\pm$ 0.03 & 0.25 $\pm$ 0.11 & 0.37 $\pm$ 0.11 & 0.28 $\pm$ 0.04 & 0.18 $\pm$ 0.05 & \cellcolor{green!10}0.07 $\pm$ 0.03 \\
        Doctor         & 0.78 $\pm$ 0.04 & 0.40 $\pm$ 0.02 & 0.50 $\pm$ 0.04 & 0.58 $\pm$ 0.03 & 0.41 $\pm$ 0.08 & \cellcolor{green!10}0.06 $\pm$ 0.01 \\
        \bottomrule
    \end{tabular}
\end{table*}

% \clearpage  % Ensures references appear separately

% \begin{refsection}
%   % supplementary text
%   \printbibliography[heading=subbibliography]
% \end{refsection}
